# Supplementary material for: Geodesic B-Score for Improved Assessment of Knee Osteoarthritis
Source: arXiv:2104.01107 ancillary file (2021-03-12)
Supplement: Supplementary file 1 [file mri_scan-ID_list.pdf]

# Geodesic B-Score for Improved Assessment of Knee Osteoarthritis

## Supplemental Material

Felix Ambellan, Stefan Zachow, and Christoph von Tycowicz

Visual and Data-centric Computing, Zuse Institute Berlin, Berlin, Germany  
{ambellan, zachow, vontycowicz}@zib.de

**Abstract.** This supplemental material features a complete list of all 9290 MRI scans from the Osteoarthritis Initiative database utilized for clinical evaluation.

### Unique MRI scan IDs defining the study population

All 3D sagittal Double Echo Steady-State MRI scans [1] were taken from the baseline time point of the Osteoarthritis Initiative<sup>1</sup> database<sup>2</sup>. In the following the IDs are given as comma separated list.

10000003, 10000011, 10000203, 10000209, 10000303, 10000309, 10000403, 10000411, 10000503, 10000509, 10000603,  
10000609, 10001503, 10001509, 10001731, 10001737, 10002103, 10002109, 10002503, 10002509, 10002703, 10002709,  
10003331, 10003337, 10003703, 10003709, 10004503, 10004509, 10004903, 10004909, 10006003, 10006009, 10006103,  
10006109, 10006203, 10006209, 10006403, 10006603, 10006609, 10006803, 10006809, 10007003, 10007009, 10007205,  
10007403, 10007409, 10009003, 10009009, 10009127, 10009133, 10009203, 10009209, 10009303, 10009309, 10009703,  
10009709, 10009803, 10009809, 10010003, 10010009, 10010321, 10010327, 10010503, 10010509, 10010629, 10010635,  
10010703, 10010709, 10010803, 10010809, 10011003, 10011009, 10011203, 10011209, 10011303, 10011309, 10011703,  
10011709, 10012003, 10012009, 10012103, 10012109, 10012503, 10012510, 10012603, 10012609, 10012703, 10012709,  
10012803, 10012809, 10012903, 10012909, 10013003, 10013009, 10013403, 10013409, 10013503, 10013509, 10013803,  
10013809, 10013903, 10013909, 10014003, 10014009, 10014131, 10014137, 10014203, 10014209, 10014403, 10014409,  
10014503, 10014509, 10014703, 10014709, 10014903, 10014909, 10015003, 10015009, 10015203, 10015209, 10015309,

---

<sup>1</sup> The Osteoarthritis Initiative is a public-private partnership comprised of five contracts (N01-AR-2-2258; N01-AR-2-2259; N01-AR-2-2260; N01-AR-2-2261; N01-AR-2-2262) funded by the National Institutes of Health, a branch of the Department of Health and Human Services, and conducted by the OAI Study Investigators. Private funding partners include Merck Research Laboratories; Novartis Pharmaceuticals Corporation, GlaxoSmithKline; and Pfizer, Inc. Private sector funding for the OAI is managed by the Foundation for the National Institutes of Health. This manuscript was prepared using an OAI public use data set and does not necessarily reflect the opinions or views of the OAI investigators, the NIH, or the private funding partners.

<sup>2</sup> [nda.nih.gov/oai](http://nda.nih.gov/oai)

10015503, 10015509, 10015703, 10015709, 10015803, 10015809, 10016103, 10016109, 10016203, 10016209, 10016309,  
 10016603, 10016609, 10016803, 10016809, 10016903, 10016911, 10017003, 10017009, 10017103, 10017109, 10017203,  
 10017209, 10017303, 10017309, 10017503, 10017509, 10017603, 10017609, 10017703, 10017709, 10017803, 10017809,  
 10018103, 10018203, 10018209, 10018303, 10018309, 10018403, 10018409, 10018510, 10018603, 10018609, 10018703,  
 10018709, 10019003, 10019009, 10019103, 10019109, 10019203, 10019209, 10019303, 10019309, 10019703, 10019709,  
 10019803, 10019809, 10020003, 10020009, 10020103, 10020109, 10020237, 10020245, 10020303, 10020309, 10020503,  
 10020509, 10020603, 10020609, 10020803, 10020809, 10020903, 10020909, 10021003, 10021011, 10021103, 10021111,  
 10021303, 10021309, 10021503, 10021509, 10021703, 10021709, 10021803, 10021809, 10022003, 10022009, 10022203,  
 10022209, 10022303, 10022309, 10022403, 10022409, 10022503, 10022509, 10022603, 10022609, 10022702, 10022708,  
 10022803, 10022809, 10022903, 10022909, 10023103, 10023109, 10023303, 10023309, 10023637, 10023645, 10024103,  
 10024109, 10024203, 10024210, 10024303, 10024309, 10024403, 10024409, 10024603, 10024733, 10024739, 10024803,  
 10024903, 10024909, 10025003, 10025009, 10025103, 10025109, 10025203, 10025209, 10025303, 10025309, 10025403,  
 10025409, 10025503, 10025509, 10025803, 10025809, 10025903, 10025909, 10026103, 10026109, 10026203, 10026209,  
 10026403, 10026409, 10026503, 10026509, 10027203, 10027209, 10027303, 10027309, 10027437, 10027503, 10027509,  
 10027803, 10027809, 10028003, 10028009, 10028303, 10028706, 10028805, 10028810, 10028906, 10029303, 10029309,  
 10029403, 10029409, 10029503, 10029509, 10029803, 10029903, 10029909, 10030005, 10030103, 10030109, 10030206,  
 10030209, 10030503, 10030509, 10030803, 10030810, 10030903, 10030909, 10031003, 10031009, 10031103, 10031109,  
 10031403, 10031409, 10031503, 10031509, 10032003, 10032009, 10032103, 10032109, 10032203, 10032209, 10032303,  
 10032309, 10032503, 10032509, 10032603, 10032609, 10032803, 10032809, 10032903, 10032909, 10033103, 10033109,  
 10033303, 10033309, 10033603, 10033609, 10033703, 10033709, 10033803, 10033809, 10033903, 10033909, 10034003,  
 10034009, 10034103, 10034109, 10034203, 10034209, 10034503, 10034509, 10034803, 10034810, 10034903, 10034909,  
 10035003, 10035009, 10035203, 10035209, 10035403, 10035409, 10035503, 10035803, 10035809, 10036104, 10036109,  
 10036218, 10036223, 10036317, 10036323, 10036417, 10036423, 10036503, 10036509, 10036703, 10036709, 10036803,  
 10036809, 10037003, 10037009, 10037103, 10037109, 10037303, 10037309, 10037403, 10037409, 10037503, 10037509,  
 10037603, 10037609, 10037803, 10037809, 10037903, 10037909, 10038303, 10038309, 10038403, 10038409, 10038617,  
 10038623, 10038703, 10038709, 10038803, 10038809, 10039009, 10039012, 10039203, 10039209, 10039503, 10039602,  
 10039609, 10039703, 10039709, 10039803, 10040103, 10040111, 10040203, 10040209, 10040303, 10040310, 10040417,  
 10040423, 10040803, 10040810, 10040903, 10040912, 10041003, 10041009, 10041117, 10041123, 10041203, 10041209,  
 10041603, 10041609, 10041803, 10041810, 10041907, 10041912, 10042103, 10042109, 10042203, 10042209, 10042303,  
 10042309, 10042403, 10042409, 10042603, 10042609, 10042803, 10042809, 10042903, 10042908, 10043106, 10043111,  
 10043603, 10043609, 10043703, 10043710, 10043803, 10043809, 10043903, 10043909, 10044010, 10044203, 10044209,  
 10044317, 10044323, 10044403, 10044409, 10044603, 10044609, 10044703, 10044709, 10044903, 10044909, 10045103,  
 10045109, 10045803, 10045902, 10045911, 10046003, 10046009, 10046103, 10046109, 10046204, 10046210, 10046503,  
 10046509, 10046603, 10046609, 10047003, 10047009, 10047103, 10047109, 10047203, 10047209, 10047303, 10047309,  
 10047403, 10047409, 10047503, 10047509, 10047703, 10047711, 10047803, 10047809, 10048103, 10048109, 10048203,  
 10048209, 10048303, 10048309, 10048418, 10048422, 10048603, 10048609, 10048803, 10048809, 10048903, 10048909,  
 10049003, 10049009, 10049103, 10049109, 10049505, 10049603, 10049609, 10049803, 10049809, 10050003, 10050009,  
 10050203, 10050209, 10050303, 10050311, 10050603, 10050609, 10050803, 10050809, 10050903, 10050909, 10051103,  
 10051109, 10051203, 10051209, 10051304, 10051309, 10051403, 10051409, 10051503, 10051513, 10051603, 10051609,  
 10051703, 10051709, 10052003, 10052008, 10052103, 10052109, 10052203, 10052210, 10052303, 10052309, 10052403,  
 10052410, 10052603, 10052609, 10052703, 10052903, 10052909, 10053005, 10053009, 10053103, 10053109, 10053303,  
 10053309, 10053703, 10053709, 10053903, 10053909, 10054003, 10054009, 10054302, 10054311, 10054403, 10054409,  
 10054603, 10054610, 10054703, 10054709, 10054803, 10054809, 10054903, 10054910, 10055005, 10055010, 10055303,  
 10055319, 10055503, 10055509, 10055903, 10055910, 10056005, 10056012, 10056103, 10056111, 10056305, 10056310,  
 10056405, 10056411, 10056605, 10056612, 10056703, 10056709, 10057103, 10057113, 10057203, 10057209, 10057303,

10057309, 10057403, 10057408, 10057548, 10057556, 10057803, 10057809, 10058003, 10058009, 10058303, 10058309, 10058503, 10058509, 10058603, 10058610, 10058703, 10058709, 10058803, 10058809, 10059004, 10059010, 10059502, 10059603, 10059609, 10059703, 10059709, 10059903, 10059909, 10060003, 10060009, 10060103, 10060109, 10060303, 10060309, 10060705, 10060711, 10060805, 10060811, 10060903, 10060909, 10061105, 10061112, 10061205, 10061211, 10061405, 10061411, 10061503, 10061509, 10061605, 10061611, 10061706, 10061727, 10061805, 10061811, 10061903, 10061909, 10062117, 10062125, 10062205, 10062211, 10062405, 10062412, 10062503, 10062512, 10062736, 10062743, 10063005, 10063011, 10063203, 10063209, 10063405, 10063413, 10063502, 10063509, 10063805, 10063811, 10063905, 10063911, 10064005, 10064011, 10064104, 10064405, 10064411, 10064506, 10064512, 10064803, 10064810, 10064907, 10064913, 10065106, 10065112, 10065321, 10065330, 10065403, 10065413, 10065506, 10065512, 10065605, 10065611, 10065706, 10065713, 10065906, 10065913, 10066003, 10066009, 10066105, 10066111, 10066403, 10066409, 10066505, 10066511, 10066617, 10066625, 10066803, 10067112, 10067305, 10067313, 10067403, 10067409, 10067523, 10067529, 10067605, 10067611, 10067705, 10067711, 10067805, 10067813, 10067905, 10067911, 10068005, 10068011, 10068105, 10068111, 10068505, 10068511, 10068605, 10068611, 10068705, 10068711, 10068805, 10068905, 10068911, 10069006, 10069012, 10069103, 10069109, 10069306, 10069312, 10069406, 10069412, 10069503, 10069603, 10069609, 10069706, 10069712, 10069803, 10069809, 10070019, 10070025, 10070203, 10070209, 10070421, 10070427, 10070504, 10070510, 10070603, 10070609, 10070906, 10070912, 10071003, 10071106, 10071112, 10071206, 10071213, 10071506, 10071512, 10071606, 10071612, 10071706, 10071712, 10071803, 10071810, 10072206, 10072212, 10072406, 10072412, 10072506, 10072512, 10072703, 10072710, 10072806, 10072812, 10072905, 10072911, 10073006, 10073012, 10073203, 10073209, 10073406, 10073412, 10073503, 10073509, 10073607, 10073613, 10073903, 10073909, 10074106, 10074112, 10074205, 10074211, 10074306, 10074312, 10074417, 10074423, 10074605, 10074611, 10074706, 10074712, 10074803, 10074809, 10074906, 10074912, 10075003, 10075010, 10075106, 10075113, 10075206, 10075212, 10075306, 10075312, 10075406, 10075412, 10075605, 10075610, 10075706, 10075712, 10075806, 10075812, 10076306, 10076406, 10076412, 10076503, 10076606, 10076613, 10076703, 10076709, 10076806, 10076812, 10076909, 10077006, 10077012, 10077103, 10077112, 10077203, 10077209, 10077303, 10077309, 10077406, 10077411, 10077612, 10077903, 10077909, 10078105, 10078111, 10078505, 10078511, 10078703, 10078709, 10078805, 10078811, 10079103, 10079109, 10079305, 10079311, 10079405, 10079411, 10079503, 10079509, 10079605, 10079611, 10079805, 10079812, 10079903, 10079909, 10080011, 10080205, 10080211, 10080303, 10080309, 10080403, 10080409, 10080503, 10080509, 10080603, 10080609, 10080703, 10080709, 10080805, 10080811, 10080903, 10080909, 10081003, 10081009, 10081105, 10081111, 10081305, 10081311, 10081405, 10081411, 10081705, 10081711, 10081805, 10081903, 10081909, 10082103, 10082109, 10082215, 10082221, 10082405, 10082415, 10082503, 10082509, 10082605, 10082611, 10082705, 10082711, 10083005, 10083011, 10083205, 10083211, 10083305, 10083311, 10083403, 10083409, 10083705, 10083711, 10083816, 10083822, 10083905, 10083911, 10084005, 10084011, 10084105, 10084111, 10084205, 10084211, 10084422, 10084432, 10084705, 10084711, 10084905, 10084911, 10085305, 10085311, 10085405, 10085410, 10085505, 10085511, 10085605, 10085611, 10085705, 10085711, 10085822, 10085828, 10086003, 10086011, 10086320, 10086326, 10086405, 10086411, 10086505, 10086511, 10086605, 10086611, 10086705, 10086711, 10087005, 10087011, 10087105, 10087115, 10087205, 10087211, 10087505, 10087511, 10087821, 10087827, 10087922, 10087928, 10088005, 10088011, 10088105, 10088111, 10088305, 10088311, 10088405, 10088414, 10088505, 10088511, 10088605, 10088611, 10088905, 10088910, 10089003, 10089103, 10089205, 10089211, 10089303, 10089309, 10089505, 10089511, 10089605, 10089614, 10089705, 10089711, 10089858, 10089863, 10090105, 10090111, 10090405, 10090411, 10090505, 10090511, 10090605, 10090611, 10090705, 10090711, 10090805, 10090811, 10090905, 10091005, 10091011, 10091105, 10091111, 10091305, 10091311, 10091405, 10091411, 10091505, 10091511, 10091805, 10091812, 10091905, 10091911, 10092105, 10092111, 10092205, 10092214, 10092305, 10092311, 10092405, 10092411, 10092517, 10092523, 10092621, 10092627, 10092705, 10092711, 10093005, 10093011, 10093303, 10093311, 10093503, 10093509, 10093606, 10093612, 10093705, 10093711, 10093906, 10093916, 10094005, 10094011, 10094405, 10094411, 10094506, 10094512, 10094805, 10094811, 10094906, 10094912, 10095106, 10095112, 10095204, 10095210, 10095405, 10095411, 10095505, 10095511, 10095605, 10095611, 10095705, 10095713, 10095805, 10095811, 10096006, 10096012,

10096106, 10096112, 10096303, 10096309, 10096506, 10096512, 10096603, 10096609, 10096706, 10096712, 10097005,  
 10097011, 10097106, 10097112, 10097205, 10097212, 10097306, 10097312, 10097405, 10097411, 10097503, 10097509,  
 10097703, 10097711, 10097805, 10097811, 10098003, 10098011, 10098306, 10098312, 10098606, 10098612, 10098703,  
 10098709, 10098806, 10098814, 10098906, 10098912, 10099406, 10099412, 10099505, 10099512, 10099706, 10099712,  
 10099806, 10099812, 10099906, 10099913, 10100906, 10100912, 10101406, 10101412, 10101706, 10101712, 10101806,  
 10101813, 10102206, 10102212, 10102420, 10102426, 10102505, 10102513, 10102606, 10102612, 10102805, 10102813,  
 10102905, 10102912, 10103006, 10103012, 10103107, 10103117, 10103206, 10103212, 10103305, 10103312, 10103505,  
 10103512, 10103903, 10104105, 10104112, 10104506, 10104512, 10104605, 10104613, 10104805, 10104816, 10105023,  
 10105029, 10105106, 10105112, 10105223, 10105229, 10105309, 10105315, 10105406, 10105413, 10105506, 10105512,  
 10105620, 10105626, 10105806, 10105814, 10105923, 10105929, 10106009, 10106017, 10106125, 10106132, 10106223,  
 10106229, 10106305, 10106312, 10106405, 10106412, 10106623, 10106629, 10106706, 10106712, 10106906, 10106912,  
 10107325, 10107331, 10107606, 10107612, 10108006, 10108012, 10108306, 10108312, 10108506, 10108512, 10108606,  
 10108612, 10108706, 10108712, 10108806, 10108812, 10109206, 10109212, 10109306, 10109312, 10109406, 10109412,  
 10109706, 10109712, 10109806, 10109812, 10109906, 10109912, 10110006, 10110012, 10110206, 10110212, 10110407,  
 10110413, 10110506, 10110512, 10110606, 10110612, 10110706, 10110906, 10110912, 10111102, 10111109, 10111206,  
 10111212, 10111406, 10111413, 10111506, 10111512, 10111606, 10111612, 10111806, 10111812, 10111903, 10112206,  
 10112212, 10112314, 10112324, 10112406, 10112412, 10112506, 10112512, 10112606, 10112612, 10112706, 10112712,  
 10112913, 10113006, 10113012, 10113106, 10113112, 10113206, 10113212, 10113303, 10113312, 10113406, 10113412,  
 10113524, 10113532, 10113606, 10113612, 10113706, 10113712, 10113906, 10113912, 10114006, 10114012, 10114105,  
 10114111, 10114305, 10114311, 10114423, 10114429, 10114605, 10114611, 10114705, 10114711, 10114803, 10114809,  
 10114905, 10114911, 10115057, 10115063, 10115105, 10115111, 10115403, 10115505, 10115511, 10115605, 10115610,  
 10115810, 10115819, 10115905, 10115911, 10116015, 10116106, 10116111, 10116205, 10116211, 10116411, 10116419,  
 10116505, 10116511, 10116606, 10116612, 10116803, 10116905, 10116911, 10117107, 10117114, 10117203, 10117209,  
 10117303, 10117405, 10117411, 10117506, 10117512, 10117603, 10117609, 10117906, 10117912, 10118006, 10118013,  
 10118103, 10118109, 10118306, 10118312, 10118430, 10118437, 10118503, 10118509, 10118606, 10118612, 10118905,  
 10118911, 10119003, 10119009, 10119105, 10119111, 10119206, 10119212, 10119305, 10119311, 10119505, 10119511,  
 10119603, 10119705, 10119711, 10119806, 10119812, 10120103, 10120109, 10120206, 10120212, 10120306, 10120312,  
 10120622, 10120630, 10120806, 10120812, 10120906, 10120912, 10121106, 10121113, 10121206, 10121212, 10121306,  
 10121312, 10121706, 10121712, 10121906, 10121912, 10122117, 10122123, 10122205, 10122213, 10122306, 10122312,  
 10122417, 10122423, 10122506, 10122513, 10122605, 10122611, 10122806, 10122812, 10122940, 10122948, 10123006,  
 10123013, 10123106, 10123112, 10123406, 10123412, 10123504, 10123624, 10123629, 10123715, 10123905, 10123911,  
 10124006, 10124012, 10124306, 10124312, 10124606, 10124612, 10124706, 10124712, 10124806, 10124812, 10124923,  
 10124929, 10125024, 10125031, 10125106, 10125112, 10125206, 10125212, 10125306, 10125312, 10125406, 10125413,  
 10125606, 10125612, 10125708, 10125713, 10125906, 10125912, 10126006, 10126012, 10126106, 10126112, 10126306,  
 10126312, 10126405, 10126411, 10126603, 10126609, 10126803, 10126810, 10126940, 10126946, 10127106, 10127112,  
 10127206, 10127213, 10127306, 10127312, 10127404, 10127411, 10127603, 10127706, 10127712, 10128106, 10128112,  
 10128206, 10128212, 10128303, 10128309, 10128406, 10128412, 10128506, 10128512, 10128606, 10128613, 10128806,  
 10128812, 10129006, 10129012, 10129106, 10129112, 10129203, 10129210, 10129320, 10129331, 10129614, 10129803,  
 10129809, 10129906, 10129912, 10130004, 10130108, 10130112, 10130203, 10130209, 10130406, 10130412, 10130506,  
 10130512, 10130606, 10130612, 10130807, 10130813, 10130903, 10130909, 10131106, 10131112, 10131203, 10131209,  
 10131305, 10131311, 10131406, 10131412, 10131606, 10131612, 10131706, 10131712, 10131806, 10131812, 10131906,  
 10131912, 10132003, 10132009, 10132107, 10132223, 10132229, 10132412, 10132506, 10132512, 10132706, 10132712,  
 10132809, 10132815, 10132906, 10132912, 10133009, 10133015, 10133106, 10133112, 10133406, 10133412, 10133506,  
 10133512, 10133706, 10133712, 10133906, 10133912, 10134006, 10134012, 10134106, 10134112, 10134206, 10134212,  
 10134306, 10134312, 10134406, 10134414, 10134506, 10134512, 10134606, 10134612, 10134806, 10134812, 10134906,

10134912, 10135103, 10135110, 10135206, 10135212, 10135303, 10135310, 10135503, 10135512, 10135903, 10135909,  
10136006, 10136014, 10136106, 10136112, 10136406, 10136414, 10136506, 10136512, 10136606, 10136612, 10136706,  
10136712, 10136806, 10136812, 10136906, 10136911, 10137106, 10137112, 10137206, 10137212, 10137323, 10137329,  
10137403, 10137409, 10137506, 10137512, 10137606, 10137612, 10137906, 10137913, 10138006, 10138106, 10138112,  
10138206, 10138212, 10138306, 10138312, 10138506, 10138514, 10138906, 10138912, 10139006, 10139012, 10139106,  
10139112, 10139208, 10139213, 10139309, 10139403, 10139409, 10139606, 10139612, 10139706, 10139712, 10139906,  
10139912, 10140006, 10140012, 10140106, 10140113, 10140206, 10140212, 10140306, 10140312, 10140406, 10140412,  
10140504, 10140513, 10140706, 10140712, 10140806, 10140812, 10141006, 10141012, 10141106, 10141112, 10141406,  
10141412, 10141506, 10141512, 10141606, 10141612, 10141706, 10141712, 10141806, 10141813, 10142006, 10142012,  
10142106, 10142112, 10142223, 10142229, 10142306, 10142312, 10142503, 10142509, 10142606, 10142612, 10142706,  
10142712, 10142805, 10142812, 10143106, 10143112, 10143205, 10143213, 10143507, 10143512, 10143606, 10143614,  
10143906, 10143912, 10144006, 10144012, 10144105, 10144112, 10144305, 10144314, 10144403, 10144410, 10144505,  
10144512, 10144606, 10144612, 10144806, 10144812, 10144906, 10144912, 10145006, 10145012, 10145106, 10145115,  
10145406, 10145412, 10145606, 10145612, 10145704, 10145712, 10145806, 10145812, 10145905, 10145913, 10146006,  
10146012, 10146102, 10146110, 10146206, 10146212, 10146305, 10146312, 10146440, 10146446, 10146605, 10146612,  
10146906, 10146912, 10147006, 10147012, 10147206, 10147212, 10147323, 10147329, 10147403, 10147506, 10147513,  
10147707, 10147712, 10147806, 10147812, 10148106, 10148112, 10148206, 10148212, 10148403, 10148506, 10148512,  
10148706, 10148712, 10148806, 10148812, 10148906, 10148912, 10149006, 10149012, 10149206, 10149213, 10149306,  
10149312, 10149406, 10149413, 10149506, 10149512, 10149606, 10149612, 10149806, 10149814, 10149906, 10149913,  
10150006, 10150012, 10150106, 10150112, 10150205, 10150606, 10150612, 10150806, 10150812, 10151006, 10151012,  
10151103, 10151206, 10151212, 10151506, 10151512, 10151606, 10151612, 10151706, 10151712, 10151806, 10151812,  
10151906, 10151912, 10152006, 10152012, 10152106, 10152112, 10152206, 10152212, 10152406, 10152412, 10152706,  
10152712, 10152806, 10152812, 10152906, 10152913, 10153006, 10153012, 10153106, 10153112, 10153306, 10153312,  
10153406, 10153412, 10153503, 10153509, 10153606, 10153612, 10153706, 10153712, 10153823, 10153829, 10153906,  
10153912, 10154006, 10154012, 10154206, 10154213, 10154306, 10154312, 10154706, 10154712, 10154806, 10154812,  
10154906, 10154912, 10155006, 10155013, 10155106, 10155113, 10155206, 10155212, 10155506, 10155512, 10155606,  
10155612, 10155706, 10155712, 10155806, 10155812, 10155906, 10155912, 10156006, 10156012, 10156206, 10156212,  
10156304, 10156506, 10156512, 10156706, 10156712, 10156806, 10156812, 10156906, 10156912, 10157006, 10157012,  
10157206, 10157212, 10157306, 10157312, 10157406, 10157412, 10157503, 10157509, 10157806, 10157812, 10158006,  
10158012, 10158223, 10158229, 10158306, 10158312, 10158406, 10158412, 10158506, 10158514, 10158606, 10158613,  
10158713, 10158906, 10158912, 10159212, 10160006, 10160012, 10160506, 10160512, 10160606, 10160612, 10160706,  
10160712, 10161106, 10161206, 10161906, 10161912, 10162007, 10162013, 10162206, 10162212, 10162306, 10162315,  
10162406, 10162412, 10162507, 10162513, 10162706, 10162712, 10162806, 10162812, 10163006, 10163013, 10163206,  
10163212, 10163306, 10163312, 10163406, 10163412, 10163507, 10163512, 10163705, 10163712, 10163806, 10163812,  
10163906, 10163912, 10164006, 10164012, 10164106, 10164112, 10164206, 10164212, 10164306, 10164312, 10164406,  
10164412, 10164706, 10164712, 10164806, 10164812, 10164923, 10164929, 10165006, 10165012, 10165106, 10165112,  
10165206, 10165213, 10165506, 10165512, 10165606, 10165612, 10165724, 10165731, 10165806, 10165812, 10165906,  
10165912, 10166106, 10166114, 10166206, 10166212, 10166406, 10166412, 10166506, 10166512, 10166606, 10166612,  
10166906, 10166912, 10167105, 10167112, 10167206, 10167212, 10167303, 10167309, 10167506, 10167512, 10167712,  
10167806, 10167812, 10167903, 10168106, 10168112, 10168205, 10168212, 10168306, 10168312, 10168906, 10168912,  
10169012, 10169106, 10169112, 10169206, 10169212, 10169307, 10169313, 10169406, 10169412, 10169506, 10169512,  
10169603, 10169609, 10169703, 10169709, 10169806, 10169812, 10169906, 10169912, 10170106, 10170112, 10170305,  
10170312, 10170406, 10170412, 10170505, 10170512, 10170606, 10170612, 10170705, 10170712, 10170806, 10170812,  
10170905, 10170912, 10171106, 10171112, 10171206, 10171212, 10171306, 10171312, 10171406, 10171413, 10171602,  
10171609, 10171805, 10171812, 10171906, 10171912, 10172106, 10172112, 10172205, 10172212, 10172306, 10172312,

10172506, 10172512, 10172605, 10172612, 10172805, 10172812, 10172906, 10172912, 10173005, 10173012, 10173106,  
 10173112, 10173403, 10173413, 10173606, 10173612, 10173706, 10173712, 10173806, 10173812, 10174006, 10174104,  
 10174206, 10174406, 10174412, 10174506, 10174512, 10174606, 10174612, 10174806, 10174813, 10174906, 10174912,  
 10175106, 10175112, 10175306, 10175312, 10175406, 10175412, 10175606, 10175612, 10175738, 10175743, 10175806,  
 10175812, 10175903, 10175909, 10176006, 10176012, 10176302, 10176310, 10176406, 10176412, 10176506, 10176512,  
 10176723, 10176729, 10176806, 10176812, 10176906, 10176912, 10177006, 10177012, 10177206, 10177212, 10177306,  
 10177312, 10177406, 10177412, 10177606, 10177612, 10177706, 10177712, 10177906, 10177912, 10178006, 10178012,  
 10178106, 10178112, 10178206, 10178212, 10178306, 10178312, 10178420, 10178426, 10178505, 10178510, 10178606,  
 10178612, 10178706, 10178712, 10178806, 10178812, 10179206, 10179213, 10179406, 10179412, 10179502, 10179509,  
 10179606, 10179612, 10179823, 10179829, 10179903, 10179909, 10180006, 10180012, 10180106, 10180112, 10180206,  
 10180212, 10180406, 10180412, 10180606, 10180612, 10180820, 10180826, 10180906, 10180912, 10181006, 10181012,  
 10181305, 10181312, 10181411, 10181418, 10181702, 10181709, 10181820, 10181826, 10181905, 10181912, 10182023,  
 10182029, 10182223, 10182229, 10182305, 10182312, 10182423, 10182429, 10182706, 10182711, 10182806, 10182812,  
 10183003, 10183009, 10183120, 10183126, 10183203, 10183323, 10183328, 10183506, 10183622, 10183629, 10183819,  
 10183824, 10183906, 10183912, 10184006, 10184206, 10184213, 10184319, 10184326, 10184423, 10184428, 10184705,  
 10184712, 10184806, 10184818, 10184905, 10184912, 10185006, 10185012, 10185206, 10185212, 10185406, 10185414,  
 10185629, 10185703, 10186005, 10186012, 10186205, 10186212, 10186307, 10186313, 10186706, 10186712, 10186805,  
 10186812, 10188306, 10188312, 10189106, 10189112, 10189206, 10189213, 10189506, 10189512, 10189720, 10189725,  
 10189806, 10189813, 10190140, 10190146, 10190203, 10190209, 10190340, 10190346, 10190506, 10190512, 10190606,  
 10190613, 10190806, 10190812, 10190909, 10190915, 10191006, 10191012, 10191120, 10191129, 10191317, 10191405,  
 10191411, 10191724, 10191730, 10191924, 10191930, 10192706, 10192712, 10192805, 10192812, 10194005, 10194012,  
 10194206, 10194212, 10194506, 10194512, 10194706, 10194712, 10195406, 10195412, 10195806, 10195812, 10196006,  
 10196012, 10196106, 10196112, 10196240, 10196246, 10196606, 10196612, 10196824, 10196831, 10197006, 10197012,  
 10197206, 10197211, 10197606, 10197612, 10197717, 10197726, 10197906, 10198406, 10198412, 10199306, 10199312,  
 10199506, 10199906, 10199912, 10200106, 10200112, 10200206, 10200212, 10200506, 10200512, 10200806, 10200812,  
 10200906, 10200912, 10201005, 10201012, 10201506, 10201512, 10201602, 10201609, 10201906, 10201912, 10202005,  
 10202012, 10202106, 10202112, 10202212, 10202306, 10202312, 10202406, 10202412, 10202506, 10202512, 10202623,  
 10202629, 10203106, 10203112, 10203206, 10203212, 10203406, 10203412, 10203507, 10203512, 10203606, 10203612,  
 10203705, 10203712, 10203806, 10203812, 10203905, 10203912, 10204305, 10204312, 10204505, 10204515, 10204703,  
 10204812, 10205206, 10205212, 10205305, 10205312, 10205406, 10205412, 10205505, 10205512, 10205606, 10205612,  
 10205905, 10205912, 10206006, 10206012, 10206105, 10206112, 10206206, 10206212, 10206303, 10206506, 10206512,  
 10206623, 10206629, 10206706, 10206712, 10206806, 10206812, 10207306, 10207312, 10207706, 10207712, 10208606,  
 10208612, 10208806, 10208812, 10209006, 10209012, 10210206, 10210212, 10210302, 10210309, 10210406, 10210412,  
 10210606, 10210612, 10210706, 10210711, 10210906, 10210912, 10211206, 10211506, 10211512, 10211706, 10211712,  
 10211805, 10211812, 10212005, 10212012, 10212412, 10212506, 10212512, 10213006, 10213012, 10213406, 10213415,  
 10213606, 10213612, 10213806, 10213812, 10214006, 10214012, 10214206, 10214212, 10214406, 10214412, 10214503,  
 10214509, 10214606, 10214704, 10214906, 10215606, 10215613, 10215706, 10215712, 10215806, 10215812, 10216106,  
 10216112, 10216223, 10216229, 10216437, 10216443, 10216640, 10216646, 10217023, 10217029, 10217123, 10217129,  
 10217206, 10217212, 10217306, 10217313, 10217506, 10217512, 10217623, 10217629, 10217706, 10217712, 10217823,  
 10217829, 10217906, 10217912, 10218006, 10218012, 10218106, 10218112, 10218223, 10218229, 10218306, 10218312,  
 10218423, 10218429, 10218527, 10218532, 10218706, 10218713, 10218807, 10218813, 10218906, 10218912, 10219005,  
 10219012, 10219106, 10219112, 10219205, 10219212, 10219405, 10219412, 10220005, 10220012, 10220205, 10220212,  
 10220406, 10220411, 10220503, 10220509, 10220708, 10220714, 10220803, 10221005, 10221012, 10221306, 10221312,  
 10221506, 10221512, 10221606, 10221612, 10221706, 10221712, 10221905, 10221912, 10222006, 10222012, 10222106,  
 10222112, 10222306, 10222312, 10222406, 10222412, 10222506, 10222512, 10222606, 10222612, 10222806, 10222812,

10222906, 10222912, 10223002, 10223009, 10223205, 10223216, 10223307, 10223313, 10223405, 10223413, 10223605,  
10223616, 10223706, 10223712, 10223805, 10223906, 10223913, 10224003, 10224010, 10224106, 10224112, 10224206,  
10224212, 10224406, 10224412, 10224506, 10224512, 10224706, 10224712, 10224806, 10224812, 10224906, 10224912,  
10225005, 10225011, 10225105, 10225111, 10225203, 10225405, 10225411, 10225505, 10225511, 10225605, 10225611,  
10225706, 10225712, 10225905, 10225911, 10226005, 10226011, 10226105, 10226111, 10226205, 10226211, 10226405,  
10226411, 10226527, 10226705, 10226711, 10226823, 10226829, 10226905, 10226911, 10227303, 10227309, 10227429,  
10227505, 10227511, 10227623, 10227630, 10227705, 10227711, 10227905, 10227911, 10228123, 10228129, 10228205,  
10228211, 10228303, 10228310, 10228405, 10228411, 10228527, 10228605, 10228611, 10229005, 10229011, 10229105,  
10229111, 10229224, 10229229, 10229506, 10229516, 10230105, 10230111, 10230305, 10230311, 10230403, 10230409,  
10230505, 10230511, 10230605, 10230611, 10231005, 10231011, 10231106, 10231114, 10231205, 10231211, 10231405,  
10231411, 10231605, 10231611, 10231706, 10231712, 10231906, 10231912, 10232005, 10232011, 10232106, 10232113,  
10232205, 10232211, 10232523, 10232529, 10232605, 10232611, 10233022, 10233027, 10233106, 10233112, 10233405,  
10233411, 10233603, 10233613, 10233805, 10233811, 10233906, 10234105, 10234111, 10234211, 10234305, 10234311,  
10234405, 10234412, 10234505, 10234511, 10234705, 10234711, 10234805, 10234811, 10234905, 10234911, 10235005,  
10235011, 10235105, 10235111, 10235206, 10235215, 10235505, 10235511, 10235705, 10235711, 10235806, 10235812,  
10235905, 10235911, 10236105, 10236112, 10236220, 10236226, 10236303, 10236309, 10236405, 10236803, 10236809,  
10236905, 10236913, 10237005, 10237014, 10237103, 10237109, 10237305, 10237311, 10237403, 10237409, 10237505,  
10237511, 10237705, 10237712, 10237803, 10237809, 10238005, 10238011, 10238105, 10238111, 10238205, 10238211,  
10238305, 10238311, 10238405, 10238411, 10238521, 10238527, 10238705, 10238711, 10239205, 10239211, 10239303,  
10239309, 10239421, 10239427, 10239523, 10239605, 10239611, 10239705, 10239711, 10239805, 10239813, 10240005,  
10240012, 10240205, 10240211, 10240305, 10240311, 10240421, 10240427, 10240505, 10240513, 10240619, 10240630,  
10240906, 10240911, 10241005, 10241011, 10241105, 10241111, 10241205, 10241211, 10241305, 10241311, 10241605,  
10241611, 10241705, 10241711, 10241805, 10241811, 10241905, 10241911, 10242006, 10242012, 10242106, 10242112,  
10242406, 10242412, 10242506, 10242512, 10242606, 10242612, 10242706, 10242712, 10242806, 10242812, 10242906,  
10242912, 10243106, 10243112, 10243206, 10243212, 10243306, 10243312, 10243406, 10243412, 10243503, 10243509,  
10243706, 10243712, 10243806, 10243812, 10244103, 10244109, 10244206, 10244212, 10244306, 10244312, 10244406,  
10244413, 10244606, 10244612, 10244706, 10244713, 10244906, 10244912, 10245006, 10245012, 10245103, 10245206,  
10245212, 10245306, 10245312, 10245503, 10245509, 10245606, 10245612, 10245907, 10245914, 10246205, 10246212,  
10246305, 10246311, 10246406, 10246412, 10246605, 10246703, 10246709, 10246806, 10246812, 10246901, 10247303,  
10247406, 10247412, 10247623, 10247630, 10247703, 10247709, 10247803, 10247809, 10248003, 10248106, 10248112,  
10248206, 10248212, 10248306, 10248312, 10248406, 10248506, 10248515, 10248606, 10248612, 10248706, 10248712,  
10248806, 10248813, 10248907, 10248912, 10249003, 10249009, 10249106, 10249112, 10249406, 10249413, 10249506,  
10249512, 10249606, 10249612, 10249703, 10249709, 10249803, 10249810, 10250006, 10250012, 10250106, 10250112,  
10250206, 10250212, 10250406, 10250412, 10250606, 10250612, 10250706, 10250712, 10250903, 10250909, 10251006,  
10251012, 10251105, 10251112, 10251206, 10251212, 10251305, 10251312, 10251406, 10251412, 10251705, 10251712,  
10251905, 10251912, 10252006, 10252012, 10252206, 10252212, 10252305, 10252313, 10252505, 10252512, 10252906,  
10252912, 10253206, 10253212, 10253406, 10253412, 10253506, 10253512, 10253606, 10253612, 10253705, 10253712,  
10253806, 10253812, 10253906, 10253912, 10254003, 10254010, 10254203, 10254306, 10254312, 10254523, 10254529,  
10254606, 10254612, 10254803, 10254809, 10254903, 10254911, 10255106, 10255112, 10255206, 10255212, 10255306,  
10255312, 10255506, 10255512, 10255603, 10255707, 10255712, 10255806, 10255812, 10256003, 10256009, 10256106,  
10256112, 10256207, 10256214, 10256306, 10256312, 10256403, 10256409, 10256506, 10256512, 10256623, 10256629,  
10256906, 10256912, 10257006, 10257012, 10257101, 10257306, 10257312, 10257406, 10257412, 10257506, 10257512,  
10257703, 10257709, 10257813, 10257906, 10257915, 10258006, 10258013, 10258102, 10258206, 10258212, 10258306,  
10258312, 10258406, 10258412, 10258506, 10258512, 10258606, 10258612, 10258706, 10258712, 10259006, 10259012,  
10259203, 10259211, 10259306, 10259312, 10259403, 10259506, 10259511, 10259606, 10259907, 10259913, 10260003,

10260009, 10260103, 10260109, 10260206, 10260212, 10260306, 10260312, 10260605, 10260703, 10260709, 10260806,  
 10260812, 10260903, 10260909, 10261006, 10261012, 10261103, 10261109, 10261203, 10261503, 10261509, 10261603,  
 10261609, 10261703, 10261709, 10261806, 10261812, 10261904, 10261909, 10262006, 10262012, 10262103, 10262109,  
 10262206, 10262212, 10262303, 10262309, 10262403, 10262409, 10262503, 10262510, 10262806, 10262812, 10263003,  
 10263009, 10263106, 10263112, 10263203, 10263209, 10263306, 10263312, 10263603, 10263609, 10263803, 10263809,  
 10263903, 10263909, 10264003, 10264009, 10264303, 10264309, 10264503, 10264509, 10264603, 10264609, 10264806,  
 10264812, 10264903, 10264909, 10265103, 10265109, 10265406, 10265412, 10265503, 10265509, 10265606, 10265612,  
 10265703, 10265709, 10265903, 10265909, 10266003, 10266009, 10266103, 10266109, 10266205, 10266211, 10266305,  
 10266313, 10266405, 10266411, 10266505, 10266511, 10266703, 10266709, 10266805, 10266813, 10266906, 10266912,  
 10267003, 10267106, 10267113, 10267206, 10267213, 10267506, 10267512, 10267606, 10267612, 10267706, 10267712,  
 10267906, 10267912, 10268006, 10268012, 10268106, 10268112, 10268323, 10268329, 10268503, 10268509, 10268603,  
 10268609, 10268706, 10268715, 10268905, 10268910, 10269103, 10269109, 10269203, 10269303, 10269309, 10269403,  
 10269412, 10269503, 10269509, 10269606, 10269614, 10269703, 10269709, 10269903, 10269909, 10270006, 10270012,  
 10270107, 10270114, 10270205, 10270212, 10270303, 10270309, 10270603, 10270609, 10270705, 10270711, 10270803,  
 10270809, 10270903, 10270909, 10271003, 10271009, 10271203, 10271209, 10271303, 10271309, 10271403, 10271409,  
 10271505, 10271511, 10271603, 10271609, 10271906, 10271912, 10272006, 10272012, 10272103, 10272109, 10272306,  
 10272312, 10272506, 10272512, 10272603, 10272610, 10272706, 10272712, 10272806, 10272812, 10272906, 10272912,  
 10273006, 10273012, 10273203, 10273209, 10273306, 10273312, 10273406, 10273412, 10273503, 10273509, 10273703,  
 10273709, 10273906, 10273912, 10274003, 10274009, 10274106, 10274112, 10274206, 10274212, 10274306, 10274312,  
 10274506, 10274512, 10274606, 10274612, 10274706, 10274712, 10274906, 10274912, 10275006, 10275012, 10275103,  
 10275306, 10275315, 10275406, 10275412, 10275506, 10275512, 10275606, 10275614, 10275706, 10275712, 10275803,  
 10275810, 10276003, 10276009, 10276103, 10276111, 10276406, 10276412, 10276506, 10276512, 10276606, 10276612,  
 10276706, 10276713, 10276806, 10276812, 10276911, 10277023, 10277029, 10277506, 10277513, 10277706, 10277712,  
 10277801, 10278203, 10278209, 10278406, 10278412, 10278606, 10278612, 10278805, 10279403, 10279409, 10279506,  
 10279512, 10279707, 10279712, 10280106, 10280115, 10281106, 10281112, 10281306, 10281312, 10281406, 10281412,  
 10281503, 10281509, 10281706, 10281712, 10281903, 10281909, 10282006, 10282013, 10282104, 10282110, 10282309,  
 10282512, 10282606, 10282612, 10282906, 10282912, 10283008, 10283203, 10283209, 10283306, 10283312, 10283406,  
 10283413, 10283506, 10283512, 10283606, 10283612, 10283706, 10283712, 10283806, 10283812, 10283906, 10283912,  
 10284006, 10284012, 10284103, 10284110, 10284303, 10284309, 10284509, 10284704, 10284709, 10284906, 10284912,  
 10285003, 10285009, 10285106, 10285112, 10285223, 10285229, 10285506, 10285512, 10285706, 10285712, 10285803,  
 10285809, 10285906, 10285912, 10286003, 10286009, 10286106, 10286112, 10286202, 10286209, 10286306, 10286312,  
 10286403, 10286409, 10286603, 10286609, 10286706, 10286712, 10286803, 10286813, 10286906, 10286912, 10287006,  
 10287012, 10287106, 10287112, 10287206, 10287212, 10287406, 10287412, 10287606, 10287612, 10287703, 10287713,  
 10287906, 10287913, 10288006, 10288012, 10288203, 10288209, 10288306, 10288312, 10288403, 10288409, 10288506,  
 10288512, 10288706, 10288712, 10288803, 10288809, 10289003, 10289009, 10289203, 10289209, 10289306, 10289312,  
 10289403, 10289603, 10289609, 10289906, 10289912, 10290006, 10290012, 10290203, 10290209, 10290403, 10290409,  
 10290506, 10290512, 10290606, 10290612, 10290706, 10290712, 10290806, 10290812, 10290906, 10290912, 10291106,  
 10291112, 10291206, 10291212, 10291406, 10291412, 10291506, 10291512, 10291603, 10291609, 10291706, 10291712,  
 10291806, 10291812, 10291906, 10291912, 10292206, 10292213, 10292406, 10292412, 10292506, 10292512, 10292706,  
 10292712, 10292906, 10292912, 10293006, 10293012, 10293106, 10293112, 10293206, 10293212, 10293303, 10293309,  
 10293606, 10293612, 10293706, 10293712, 10293806, 10293812, 10293906, 10293912, 10294103, 10294109, 10294306,  
 10294312, 10294606, 10294612, 10294706, 10294712, 10294806, 10294814, 10294903, 10295006, 10295012, 10295106,  
 10295112, 10295203, 10295506, 10295512, 10295706, 10295712, 10295806, 10295812, 10295906, 10295912, 10296106,  
 10296112, 10296205, 10296216, 10296303, 10296309, 10296606, 10296617, 10296706, 10296712, 10296905, 10296916,  
 10297006, 10297012, 10297105, 10297112, 10297206, 10297212, 10297322, 10297329, 10297405, 10297412, 10297505,



10297512, 10297606, 10297612, 10297706, 10297712, 10297906, 10297912, 10298002, 10298012, 10298306, 10298312, 10298405, 10298412, 10298506, 10298512, 10298606, 10298612, 10298706, 10298712, 10298906, 10298912, 10299006, 10299012, 10299306, 10299312, 10299403, 10299409, 10299505, 10299516, 10299801, 10299906, 10299913, 10300106, 10300111, 10300401, 10300503, 10300606, 10300612, 10300806, 10300812, 10300906, 10300912, 10301006, 10301012, 10301106, 10301112, 10301206, 10301212, 10301306, 10301312, 10301506, 10301514, 10301640, 10301646, 10301703, 10301709, 10301806, 10301814, 10301906, 10301912, 10302003, 10302010, 10302106, 10302113, 10302324, 10302330, 10302406, 10302506, 10302512, 10302806, 10302812, 10302905, 10302912, 10303006, 10303012, 10303305, 10303312, 10303406, 10303412, 10303505, 10303512, 10303606, 10303612, 10303705, 10303712, 10303806, 10303812, 10303905, 10303912, 10304102, 10304109, 10304206, 10304212, 10304302, 10304309, 10304406, 10304412, 10304505, 10304512, 10304605, 10304612, 10304805, 10304812, 10305106, 10305112, 10305205, 10305212, 10305306, 10305312, 10305506, 10305512, 10305603, 10305805, 10305812, 10305906, 10305912, 10306005, 10306012, 10306106, 10306112, 10306222, 10306229, 10306422, 10306429, 10306506, 10306512, 10306706, 10306712, 10306805, 10306812, 10306905, 10306911, 10307005, 10307012, 10307406, 10307412, 10307506, 10307514, 10307702, 10307709, 10307806, 10307812, 10307902, 10307909, 10308202, 10308211, 10308306, 10308312, 10308403, 10308410, 10308506, 10308512, 10308706, 10308712, 10308802, 10308809, 10308903, 10308910, 10309106, 10309112, 10309209, 10309323, 10309329, 10309405, 10309602, 10309609, 10309706, 10309712, 10309802, 10309809, 10309906, 10309912, 10310002, 10310009, 10310106, 10310112, 10310202, 10310209, 10310505, 10310606, 10310612, 10310706, 10310712, 10310806, 10310812, 10311005, 10311012, 10311105, 10311116, 10311205, 10311212, 10311302, 10311309, 10311507, 10311512, 10311705, 10311712, 10311909, 10312005, 10312012, 10312205, 10312210, 10312406, 10312412, 10312505, 10312513, 10312706, 10312712, 10312806, 10312812, 10313006, 10313012, 10313106, 10313112, 10313202, 10313209, 10313306, 10313312, 10313506, 10313512, 10313706, 10313712, 10313907, 10313913, 10314106, 10314112, 10314203, 10314210, 10314306, 10314312, 10314403, 10314408, 10314603, 10314609, 10314706, 10314712, 10314906, 10314912, 10315003, 10315008, 10315106, 10315112, 10315203, 10315209, 10315306, 10315312, 10315403, 10315409, 10315506, 10315512, 10315806, 10315812, 10315907, 10315913, 10316003, 10316009, 10316105, 10316112, 10316206, 10316212, 10316606, 10316612, 10316709, 10316806, 10316812, 10316905, 10316913, 10317302, 10317406, 10317412, 10317606, 10317612, 10317706, 10317712, 10317806, 10317812, 10317906, 10317912, 10318006, 10318012, 10318106, 10318112, 10318206, 10318212, 10318406, 10318412, 10318506, 10318512, 10319306, 10319312, 10319506, 10319514, 10319706, 10319712, 10319906, 10319912, 10320006, 10320012, 10320105, 10320114, 10320505, 10320514, 10321006, 10321012, 10321105, 10321112, 10321206, 10321212, 10321305, 10321312, 10321605, 10321612, 10321702, 10321709, 10321906, 10321914, 10322106, 10322115, 10322206, 10322212, 10322306, 10322312, 10322406, 10322412, 10322606, 10322612, 10322706, 10322712, 10322906, 10322913, 10323006, 10323012, 10323106, 10323114, 10323206, 10323212, 10323305, 10323312, 10323403, 10323409, 10323505, 10323513, 10323606, 10323612, 10323902, 10323912, 10324102, 10324109, 10324206, 10324212, 10324406, 10324412, 10324516, 10324523, 10324606, 10324612, 10324705, 10324712, 10324823, 10324829, 10325006, 10325012, 10325106, 10325112, 10325206, 10325212, 10325405, 10325412, 10325706, 10325712, 10325805, 10325815, 10325903, 10325909, 10326006, 10326012, 10326206, 10326212, 10326406, 10326414, 10326503, 10326509, 10326706, 10326712, 10326806, 10326814, 10327006, 10327013, 10327106, 10327113, 10327306, 10327312, 10327406, 10327413, 10327505, 10327606, 10327612, 10327706, 10327712, 10328005, 10328012, 10328106, 10328112, 10328207, 10328214, 10328306, 10328314, 10328506, 10328512, 10328604, 10328706, 10328712, 10328805, 10328813, 10328906, 10328912, 10329003, 10329009, 10329206, 10329214, 10329406, 10329412, 10329805, 10329812, 10330005, 10330012, 10330106, 10330112, 10330222, 10330229, 10330303, 10330403, 10330925, 10330932, 10331406, 10331413, 10331706, 10331712, 10332003, 10332105, 10332112, 10332206, 10332212, 10332406, 10332412, 10332712, 10332806, 10332812, 10332906, 10332912, 10333202, 10333507, 10333513, 10333706, 10333712, 10333805, 10333812, 10333906, 10333912, 10334205, 10334212, 10334405, 10334412, 10334605, 10334612, 10334805, 10334812, 10334905, 10335006, 10335012, 10335106, 10335112, 10335205, 10335212, 10335306, 10335312, 10335603, 10335824, 10335831, 10335906, 10335912, 10336005, 10336012, 10336106, 10336114, 10336205, 10336212, 10336309, 10336723, 10336729, 10336805, 10336813, 10336906, 10336912, 10337003,

10337009, 10337306, 10337312, 10337406, 10337413, 10337503, 10337512, 10337706, 10337712, 10337903, 10338006,  
 10338014, 10338106, 10338112, 10338406, 10338412, 10338506, 10338512, 10338606, 10338612, 10338706, 10338712,  
 10338803, 10338809, 10338906, 10338912, 10339006, 10339012, 10339106, 10339112, 10339206, 10339212, 10339306,  
 10339312, 10339406, 10339412, 10339706, 10339712, 10339806, 10339812, 10340006, 10340012, 10340106, 10340112,  
 10340306, 10340312, 10340406, 10340412, 10340606, 10340612, 10340706, 10340712, 10340806, 10340812, 10340906,  
 10340912, 10341106, 10341112, 10341206, 10341212, 10341306, 10341312, 10341403, 10341409, 10341506, 10341513,  
 10341606, 10341612, 10341903, 10341910, 10342006, 10342012, 10342106, 10342113, 10342206, 10342212, 10342306,  
 10342313, 10342406, 10342412, 10342506, 10342512, 10342623, 10342629, 10342806, 10342812, 10342906, 10342912,  
 10343240, 10343246, 10343306, 10343312, 10343403, 10343409, 10343506, 10343512, 10343606, 10343612, 10343706,  
 10343714, 10343806, 10343812, 10343906, 10343912, 10347006, 10347012, 10347206, 10347213, 10347403, 10347409,  
 10347806, 10347814, 10348006, 10348012, 10348223, 10348229, 10348405, 10348412, 10348605, 10348616, 10348809,  
 10348814, 10349005, 10349012, 10349205, 10349212, 10350106, 10350112, 10350423, 10350429, 10350505, 10350512,  
 10350606, 10350612, 10350705, 10350806, 10350813, 10350906, 10350912, 10351015, 10351106, 10351112, 10351206,  
 10351212, 10351405, 10351417, 10351545, 10351551, 10351707, 10351713, 10351805, 10351812, 10352106, 10352112,  
 10352205, 10352212, 10352306, 10352315, 10352405, 10352412, 10352906, 10352913, 10374006, 10374012, 10374506,  
 10374512, 10374606, 10374806, 10374812, 10375006, 10375012, 10375105, 10375112, 10375506, 10375512, 10375606,  
 10375612, 10375706, 10375806, 10375812, 10375906, 10375911, 10376106, 10376112, 10376206, 10376212, 10376406,  
 10376412, 10376706, 10376712, 10376806, 10376814, 10376923, 10376929, 10377205, 10377212, 10377306, 10377312,  
 10377506, 10377512, 10377612, 10377805, 10377813, 10378005, 10378012, 10378106, 10378112, 10378212, 10378306,  
 10378312, 10378506, 10378512, 10378706, 10378714, 10378806, 10378813, 10378906, 10378912, 10379112, 10379206,  
 10379213, 10379606, 10379612, 10379706, 10379712, 10379806, 10379812, 10379906, 10379912, 10380006, 10380012,  
 10380306, 10380312, 10380506, 10380512, 10380706, 10380712, 10380806, 10380812, 10381009, 10381013, 10381106,  
 10381112, 10381206, 10381213, 10381406, 10381412, 10381606, 10381612, 10381706, 10381712, 10381806, 10381811,  
 10382022, 10382029, 10382205, 10382212, 10382305, 10382314, 10382406, 10382413, 10382505, 10382514, 10382605,  
 10382612, 10382906, 10383023, 10383028, 10383106, 10383112, 10383340, 10383347, 10383406, 10383412, 10383506,  
 10383512, 10383606, 10383612, 10383723, 10383730, 10383806, 10383812, 10383906, 10383912, 10384006, 10384012,  
 10384106, 10384112, 10384306, 10384312, 10384557, 10384563, 10384806, 10384812, 10384905, 10384912, 10385206,  
 10385212, 10385306, 10385312, 10385506, 10385513, 10385906, 10385912, 10386306, 10386312, 10386406, 10386412,  
 10386503, 10386509, 10386905, 10386912, 10387006, 10387012, 10387105, 10387112, 10387406, 10387412, 10387505,  
 10387513, 10387705, 10387713, 10387905, 10387912, 10388103, 10388206, 10388212, 10388305, 10388312, 10388606,  
 10388612, 10388905, 10388912, 10389106, 10389112, 10389306, 10389311, 10389923, 10389929, 10390107, 10390112,  
 10390306, 10390311, 10390806, 10390812, 10391406, 10391412, 10391540, 10391546, 10391606, 10391612, 10391706,  
 10391712, 10392225, 10392232, 10392306, 10392312, 10392406, 10392412, 10392506, 10392512, 10392612, 10393305,  
 10393312, 10393505, 10393512, 10393606, 10393612, 10393702, 10393709, 10394105, 10394113, 10394305, 10394312,  
 10394705, 10394713, 10395006, 10395012, 10395206, 10395212, 10395306, 10395312, 10395505, 10395512, 10396105,  
 10396112, 10396305, 10396312, 10396705, 10396712, 10396831, 10396905, 10396912, 10397105, 10397112, 10397206,  
 10397212, 10397322, 10397329, 10397406, 10397412, 10397605, 10397612, 10397905, 10397911, 10398003, 10398303,  
 10398309, 10398406, 10398412, 10398506, 10398512, 10398806, 10398812, 10398906, 10398912, 10399206, 10399406,  
 10399415, 10399506, 10399512, 10399606, 10399612, 10399806, 10399812, 10400006, 10400012, 10400206, 10400212,  
 10400306, 10400312, 10400518, 10400524, 10400623, 10400629, 10400806, 10400812, 10401106, 10401112, 10401306,  
 10401312, 10401406, 10401412, 10401706, 10401713, 10401806, 10401813, 10401909, 10402006, 10402012, 10402206,  
 10402212, 10402406, 10402412, 10402506, 10402512, 10402603, 10402609, 10402706, 10402713, 10402806, 10402812,  
 10402906, 10402912, 10403003, 10403405, 10403412, 10403625, 10403630, 10403705, 10403713, 10403805, 10403812,  
 10403905, 10403912, 10404206, 10404212, 10404306, 10404312, 10404406, 10404412, 10405023, 10405029, 10405106,  
 10405112, 10405506, 10405513, 10405806, 10405813, 10406023, 10406029, 10406106, 10406112, 10406206, 10406212,

10406305, 10406311, 10406406, 10406412, 10406506, 10406513, 10406623, 10406629, 10406723, 10406729, 10407006,  
10407013, 10407406, 10407412, 10407506, 10407512, 10407606, 10407612, 10407705, 10407712, 10407906, 10407912,  
10408105, 10408113, 10408206, 10408212, 10408305, 10408313, 10408406, 10408412, 10408606, 10408611, 10409006,  
10409012, 10409123, 10409129, 10409206, 10409212, 10409806, 10409812, 10410022, 10410029, 10410223, 10410231,  
10410306, 10410312, 10410506, 10410512, 10410606, 10410612, 10410706, 10410712, 10410806, 10410812, 10411006,  
10411012, 10411206, 10411212, 10411306, 10411312, 10411406, 10411412, 10411506, 10411512, 10411706, 10411712,  
10411906, 10411912, 10412106, 10412112, 10412213, 10412306, 10412312, 10412406, 10412412, 10412506, 10412512,  
10412912, 10413106, 10413112, 10413406, 10413412, 10414006, 10414012, 10414106, 10414112, 10414306, 10414312,  
10414706, 10414712, 10414805, 10414812, 10414906, 10414912, 10415009, 10415013, 10415506, 10415512, 10416306,  
10416312, 10416405, 10416412, 10416606, 10416612, 10416906, 10416912, 10417006, 10417012, 10417106, 10417206,  
10417212, 10417306, 10417312, 10417705, 10417712, 10417806, 10417812, 10418305, 10418312, 10418406, 10418412,  
10418507, 10418512, 10418705, 10418712, 10418806, 10418812, 10418905, 10418912, 10419006, 10419012, 10419206,  
10419212, 10419506, 10419512, 10419706, 10419712, 10419806, 10419812, 10420006, 10420012, 10420206, 10420212,  
10420306, 10420312, 10420407, 10420413, 10420606, 10420612, 10420706, 10420712, 10421006, 10421012, 10421106,  
10421112, 10421206, 10421212, 10421506, 10421512, 10421625, 10421636, 10421823, 10421829, 10421906, 10421912,  
10422006, 10422012, 10422108, 10422112, 10422702, 10422709, 10422905, 10422912, 10423314, 10423406, 10423412,  
10423507, 10423513, 10423705, 10423712, 10423906, 10423916, 10424206, 10424212, 10424405, 10424412, 10424605,  
10424613, 10424805, 10424812, 10425023, 10425029, 10425106, 10425112, 10425206, 10425212, 10425306, 10425312,  
10425406, 10425412, 10425706, 10425712, 10425923, 10425929, 10426205, 10426212, 10426306, 10426312, 10426506,  
10426512, 10426605, 10426612, 10426812, 10426906, 10426913, 10427005, 10427012, 10427106, 10427112, 10427205,  
10427212, 10427706, 10427714, 10427805, 10427812, 10428006, 10428012, 10428106, 10428112, 10428206, 10428212,  
10428306, 10428312, 10428506, 10428512, 10428606, 10428612, 10428823, 10428829, 10428906, 10428912, 10429006,  
10429012, 10429125, 10429133, 10429403, 10429606, 10429612, 10429706, 10429712, 10429806, 10429812, 10430206,  
10430213, 10430506, 10430512, 10430706, 10430712, 10431006, 10431012, 10431103, 10431206, 10431213, 10431406,  
10431412, 10431505, 10431513, 10431606, 10431612, 10431705, 10431712, 10431807, 10431813, 10431905, 10431912,  
10432006, 10432012, 10432206, 10432212, 10433005, 10433012, 10433106, 10433112, 10433306, 10433312, 10433506,  
10433512, 10433606, 10433612, 10433806, 10433812, 10434006, 10434012, 10434206, 10434212, 10434506, 10434513,  
10434606, 10434612, 10434712, 10434906, 10434912, 10435106, 10435112, 10435207, 10435213, 10435306, 10435312,  
10435603, 10435704, 10436106, 10436112, 10436205, 10436212, 10436605, 10436612, 10436706, 10436712, 10436805,  
10436812, 10436924, 10436931, 10437406, 10437412, 10437506, 10437512, 10437806, 10437814, 10437903, 10437909,  
10438007, 10438013, 10438305, 10438312, 10438505, 10438512, 10438606, 10438613, 10438702, 10438709, 10438806,  
10438812, 10439206, 10439212, 10439408, 10439413, 10439705, 10439712, 10439905, 10439912, 10440206, 10440212,  
10440606, 10440612, 10440806, 10440812, 10441024, 10441031, 10441106, 10441112, 10441207, 10441606, 10441612,  
10442006, 10442012, 10442106, 10442112, 10442206, 10442212, 10442306, 10442312, 10442406, 10442412, 10442803,  
10442809, 10443006, 10443012, 10443206, 10443212, 10443305, 10443312, 10443606, 10443612, 10443705, 10443712,  
10443804, 10444006, 10444012, 10444105, 10444112, 10444306, 10444312, 10444406, 10444412, 10444505, 10444512,  
10444606, 10444612, 10445105, 10445112, 10445406, 10445412, 10445606, 10445612, 10445806, 10445812, 10445903,  
10446003, 10446106, 10446116, 10446206, 10446213, 10446506, 10446512, 10446906, 10446913, 10447003, 10447106,  
10447112, 10447406, 10447412, 10447806, 10447812, 10447906, 10447912, 10448306, 10448312, 10448406, 10448412,  
10448506, 10448512, 10448606, 10448612, 10449005, 10449012, 10449206, 10449212, 10449505, 10449512, 10449705,  
10449713, 10449905, 10449912, 10450003, 10450009, 10450206, 10450212, 10450305, 10450312, 10450406, 10450412,  
10450705, 10450712, 10450806, 10450812, 10450905, 10450912, 10451206, 10451212, 10451305, 10451313, 10451702,  
10451709, 10451806, 10451812, 10451907, 10451913, 10452305, 10452312, 10452406, 10452412, 10452606, 10452612,  
10452706, 10452906, 10452912, 10453006, 10453012, 10453106, 10453112, 10453206, 10453212, 10453307, 10453315,  
10453808, 10454205, 10454212, 10454705, 10454712, 10454805, 10454812, 10454905, 10454913, 10455206, 10455212,

10455306, 10455313, 10455406, 10455412, 10455509, 10455515, 10455706, 10455715, 10455806, 10455813, 10456022,  
 10456206, 10456212, 10456406, 10456412, 10456506, 10456512, 10456703, 10456806, 10456812, 10456906, 10456912,  
 10457106, 10457112, 10457306, 10457312, 10457506, 10457512, 10457606, 10457612, 10457706, 10457712, 10458106,  
 10458112, 10458206, 10458212, 10458306, 10458312, 10458406, 10458414, 10458706, 10458712, 10458806, 10458812,  
 10458906, 10458912, 10459106, 10459112, 10459406, 10459411, 10459606, 10459612, 10459706, 10459712, 10459823,  
 10459832, 10460006, 10460012, 10460206, 10460212, 10460306, 10460312, 10460406, 10460412, 10460706, 10461606,  
 10461612, 10461706, 10461712, 10462606, 10462612, 10462706, 10462712, 10462806, 10462812, 10462906, 10462912,  
 10463106, 10463112, 10463206, 10463212, 10463606, 10463612, 10463806, 10463812, 10463906, 10463912, 10464106,  
 10464112, 10464306, 10464312, 10465205, 10465306, 10465312, 10465405, 10465412, 10465805, 10465812, 10466005,  
 10466012, 10466605, 10466616, 10467106, 10467112, 10467306, 10467312, 10467506, 10467512, 10467605, 10467612,  
 10467805, 10467812, 10468002, 10468009, 10468106, 10468112, 10468205, 10468212, 10468306, 10468312, 10468405,  
 10468413, 10468508, 10468706, 10468712, 10468805, 10468812, 10469006, 10469012, 10469606, 10469612, 10470105,  
 10470112, 10470206, 10470212, 10470505, 10470512, 10470606, 10470612, 10470803, 10470809, 10470905, 10470912,  
 10471105, 10471112, 10471206, 10471212, 10471406, 10471412, 10471505, 10471512, 10471606, 10471612, 10472206,  
 10472212, 10472512, 10472706, 10472712, 10472906, 10472912, 10473103, 10473109, 10473205, 10473212, 10473306,  
 10473312, 10473506, 10473513, 10473806, 10473812, 10473906, 10473912, 10474006, 10474012, 10474112, 10474206,  
 10474212, 10474406, 10474412, 10474515, 10474906, 10474912, 10475020, 10475026, 10475206, 10475211, 10475306,  
 10475312, 10475506, 10475512, 10475606, 10475612, 10475706, 10475712, 10475812, 10475906, 10475912, 10476103,  
 10476111, 10476319, 10476325, 10476506, 10476512, 10476960, 10476967, 10477306, 10477312, 10477806, 10477812,  
 10478306, 10478312, 10478606, 10478612, 10479106, 10479112, 10479605, 10479612, 10480025, 10480032, 10480106,  
 10480112, 10480506, 10480512, 10480807, 10480812, 10480908, 10480913, 10481106, 10481112, 10481223, 10481229,  
 10481306, 10481312, 10481623, 10481629, 10481706, 10481712, 10481806, 10481813, 10482227, 10482233, 10482506,  
 10482512, 10482606, 10482612, 10482706, 10482712, 10482906, 10482912, 10483106, 10483112, 10483206, 10483212,  
 10483406, 10483415, 10483506, 10483513, 10483606, 10483612, 10483706, 10483712, 10484006, 10484013, 10484106,  
 10484207, 10484213, 10484406, 10484412, 10484606, 10484612, 10484706, 10484712, 10484806, 10484813, 10484906,  
 10484913, 10485006, 10485012, 10485206, 10485212, 10485306, 10485312, 10485403, 10485409, 10485606, 10485612,  
 10485906, 10485912, 10486106, 10486113, 10486306, 10486312, 10486605, 10486612, 10486706, 10486712, 10487005,  
 10487012, 10487202, 10487210, 10487306, 10487313, 10487405, 10487412, 10487605, 10487612, 10488303, 10488506,  
 10488512, 10489306, 10489312, 10489403, 10489506, 10489513, 10489605, 10489612, 10489805, 10489812, 10489906,  
 10489912, 10490106, 10490112, 10490205, 10490212, 10490307, 10490312, 10490406, 10490412, 10490506, 10490512,  
 10490605, 10490612, 10490906, 10490912, 10491006, 10491012, 10491206, 10491212, 10491407, 10491414, 10491506,  
 10491512, 10491604, 10491706, 10491712, 10491906, 10491912, 10492106, 10492112, 10492206, 10492215, 10492606,  
 10492612, 10492906, 10492912, 10493003, 10493105, 10493112, 10493206, 10493212, 10493306, 10493312, 10493506,  
 10493906, 10493914, 10494306, 10494313, 10494406, 10494412, 10494506, 10494512, 10494806, 10494812, 10495106,  
 10495112, 10495206, 10495212, 10495806, 10495812, 10495906, 10495912, 10496206, 10496212, 10496306, 10496312,  
 10496506, 10496512, 10496906, 10496912, 10497006, 10497014, 10497105, 10497113, 10497406, 10497412, 10498106,  
 10498112, 10498205, 10498212, 10498405, 10498412, 10498805, 10498812, 10499405, 10499412, 10499706, 10499712,  
 10499806, 10499812, 10500006, 10500013, 10500805, 10500812, 10501403, 10502023, 10502029, 10502306, 10502312,  
 10502406, 10502412, 10502606, 10502612, 10502706, 10502712, 10503006, 10503012, 10504306, 10504312, 10504506,  
 10504512, 10504606, 10504612, 10504706, 10504712, 10504806, 10504812, 10505106, 10505112, 10505606, 10505612,  
 10505706, 10505712, 10505816, 10505905, 10505912, 10506106, 10506112, 10506312, 10506318, 10506606, 10506613,  
 10507606, 10507612, 10508106, 10508112, 10508206, 10508212, 10508506, 10508515, 10508706, 10508712, 10508906,  
 10508912, 10509302, 10509309, 10509705, 10509712, 10510006, 10510012, 10510106, 10510113, 10510206, 10510212,  
 10510403, 10510506, 10510512, 10511106, 10511112, 10511306, 10511312, 10511623, 10511629, 10511706, 10511712,  
 10511806, 10511812, 10512106, 10512112, 10512404, 10515106, 10515112, 10515312, 10515406, 10515413, 10515606,

10515612, 10515806, 10515812, 10516506, 10516512, 10516806, 10516812, 10517106, 10517112, 10517206, 10517212, 10517706, 10517713, 10517803, 10517906, 10517912, 10518105, 10518112, 10518705, 10518712, 10518806, 10518812, 10518905, 10518912, 10519105, 10519113, 10519505, 10519512, 10519622, 10519629, 10519705, 10519712, 10519905, 10519912, 10520005, 10520012, 10520305, 10520312, 10520505, 10520512, 10520705, 10520712, 10520903, 10524006, 10524012, 10524105, 10524113, 10524203, 10524209, 10524305, 10524312, 10524406, 10524412, 10524606, 10524612, 10524806, 10524813, 10525207, 10525212, 10525406, 10525413, 10525606, 10525612, 10525806, 10525812, 10526005, 10526012, 10526205, 10526212, 10526605, 10526613, 10527106, 10527112, 10527206, 10527212, 10527306, 10527312, 10527406, 10527414, 10527706, 10527712, 10527806, 10527812, 10527912, 10528006, 10528012, 10528107, 10528113, 10528206, 10528213, 10528323, 10528330, 10528605, 10528612, 10528705, 10528712, 10528805, 10528812, 10529302, 10529405, 10529412, 10529502, 10529722, 10529729, 10529905, 10529912, 10530206, 10530212, 10530513, 10530606, 10530612, 10530806, 10530811, 10530906, 10530912, 10531006, 10531012, 10531141, 10531149, 10531320, 10531329, 10531402, 10531409, 10531506, 10531512, 10531602, 10531612, 10531702, 10531709, 10532206, 10532213, 10532506, 10532512, 10532703, 10532709, 10532906, 10532912, 10533006, 10533012, 10533224, 10533230, 10533306, 10533312, 10533506, 10533512, 10533706, 10533712, 10534106, 10534112, 10534306, 10534311, 10534423, 10534429, 10534506, 10534512, 10534706, 10534714, 10535023, 10535029, 10535106, 10535112, 10535506, 10535512, 10535806, 10535812, 10535906, 10535912, 10536006, 10536012, 10536106, 10536112, 10536206, 10536212, 10536406, 10536412, 10536506, 10536512, 10536706, 10536712, 10536840, 10536846, 10536906, 10536912, 10537006, 10537012, 10537206, 10537213, 10537403, 10537502, 10537511, 10537606, 10537615, 10537706, 10537712, 10537806, 10537812, 10537905, 10537912, 10538102, 10538110, 10538405, 10538412, 10538606, 10538612, 10538705, 10538712, 10538811, 10538905, 10538912, 10539006, 10539012, 10539305, 10539312, 10539522, 10539529, 10539606, 10539612, 10539806, 10539812, 10539905, 10539912, 10540006, 10540012, 10540206, 10540212, 10540305, 10540312, 10540505, 10540512, 10540606, 10540614, 10540705, 10540713, 10541106, 10541115, 10541406, 10541412, 10541506, 10541512, 10541606, 10541615, 10541706, 10541712, 10541806, 10541812, 10541906, 10541912, 10542205, 10542212, 10542306, 10542405, 10542412, 10542506, 10542512, 10542605, 10542612, 10542706, 10542712, 10542806, 10542906, 10542912, 10543206, 10543303, 10543406, 10543412, 10543506, 10543513, 10543613, 10543706, 10543713, 10544040, 10544046, 10544206, 10544212, 10544406, 10544412, 10544606, 10544612, 10544706, 10544712, 10545105, 10545112, 10545206, 10545212, 10545305, 10545312, 10545506, 10545512, 10545706, 10545712, 10545806, 10545812, 10545906, 10545913, 10546106, 10546112, 10546212, 10546306, 10546313, 10546405, 10546412, 10546612, 10546708, 10546714, 10546803, 10546912, 10547106, 10547112, 10547205, 10547212, 10547306, 10547312, 10547506, 10547512, 10547605, 10547612, 10547723, 10547729, 10547805, 10547812, 10548006, 10548012, 10548506, 10548512, 10548606, 10548612, 10548706, 10548712, 10548806, 10548812, 10548923, 10548929, 10549006, 10549012, 10549105, 10549112, 10549206, 10549212, 10549305, 10549312, 10549423, 10549429, 10549705, 10549712, 10549806, 10549812, 10550305, 10550312, 10550406, 10550412, 10550505, 10550512, 10550606, 10550612, 10550703, 10550802, 10550809, 10550905, 10550912, 10551006, 10551012, 10551106, 10551305, 10551312, 10551406, 10551412, 10551505, 10551512, 10551704, 10551710, 10552006, 10552012, 10552505, 10552512, 10552613, 10552913, 10553006, 10553013, 10553106, 10553306, 10553312, 10554106, 10554112, 10554205, 10554212, 10554405, 10554412, 10554606, 10554612, 10554806, 10554812, 10554906, 10554912, 10555006, 10555012, 10555106, 10555112, 10555403, 10555411, 10555603, 10555609, 10555706, 10555712, 10555806, 10555812, 10556006, 10556014, 10556407, 10556415, 10556506, 10556512, 10556606, 10556612, 10556806, 10556812, 10557006, 10557012, 10557106, 10557112, 10557206, 10557212, 10557306, 10557312, 10557506, 10557512, 10557706, 10557712, 10557830, 10557843, 10557923, 10557929, 10558206, 10558212, 10558305, 10558312, 10558406, 10558412, 10558505, 10558512, 10558606, 10558612, 10558803, 10558809, 10558905, 10558912, 10559005, 10559012, 10559205, 10559216, 10559322, 10559329, 10559505, 10559514, 10559805, 10559812, 10559905, 10559912, 10560105, 10560112, 10560413, 10560506, 10560511, 10560606, 10560612, 10560909, 10561003, 10561009, 10561106, 10561112, 10561206, 10561212, 10561606, 10561612, 10562206, 10562212, 10562306, 10562406, 10562413, 10562706, 10562713, 10562806, 10562812, 10562907, 10562913, 10563006, 10563206, 10563212, 10563306, 10563312, 10563805, 10563812, 10564005, 10564014, 10564106, 10564112,

10564206, 10564212, 10564523, 10564532, 10564606, 10564612, 10564706, 10564712, 10564906, 10564912, 10565206,  
 10565212, 10565406, 10565412, 10565706, 10565712, 10565924, 10565930, 10566005, 10566012, 10566103, 10566109,  
 10566205, 10566212, 10566422, 10566429, 10566506, 10566512, 10566605, 10566612, 10566802, 10566809, 10567106,  
 10567112, 10567405, 10567412, 10567506, 10567512, 10567605, 10567613, 10567703, 10567903, 10567909, 10568006,  
 10568012, 10568148, 10568154, 10568309, 10568315, 10568606, 10568612, 10568805, 10568811, 10569006, 10569012,  
 10569107, 10569112, 10569206, 10569213, 10569323, 10569329, 10569406, 10569412, 10569506, 10569512, 10569705,  
 10569712, 10569805, 10569813, 10570005, 10570014, 10570105, 10570112, 10570405, 10570412, 10570822, 10570829,  
 10571106, 10571113, 10571205, 10571212, 10571408, 10571415, 10571706, 10571712, 10571806, 10571814, 10571906,  
 10571912, 10572006, 10572011, 10572106, 10572112, 10572306, 10572312, 10572406, 10572412, 10572806, 10572812,  
 10573006, 10573012, 10573106, 10573112, 10573206, 10573212, 10573306, 10573312, 10573602, 10573609, 10573706,  
 10573711, 10574105, 10574112, 10574205, 10574212, 10574405, 10574412, 10574505, 10574512, 10574607, 10574615,  
 10574805, 10574812, 10575206, 10575212, 10575406, 10575412, 10575606, 10575612, 10575706, 10575712, 10575806,  
 10575812, 10576006, 10576012, 10576106, 10576112, 10576406, 10576412, 10576506, 10576512, 10576806, 10576812,  
 10577106, 10577112, 10577306, 10577312, 10577506, 10577512, 10578806, 10578812, 10578906, 10578912, 10579106,  
 10579112, 10579206, 10579212, 10579306, 10579312, 10579606, 10579614, 10579706, 10579712, 10579834, 10579840,  
 10579906, 10579913, 10580106, 10580112, 10580223, 10580229, 10580306, 10580312, 10580506, 10580512, 10580708,  
 10581005, 10581012, 10581405, 10581412, 10581506, 10581512, 10581805, 10581812, 10582807, 10582813, 10583103,  
 10583109, 10583506, 10583512, 10583607, 10583613, 10583906, 10583912, 10584106, 10584112, 10584507, 10584513,  
 10584603, 10584806, 10585306, 10585312, 10585405, 10585412, 10586103, 10586109, 10586306, 10586312, 10586507,  
 10586513, 10586605, 10586612, 10586805, 10586813, 10586905, 10586912, 10587006, 10587012, 10587406, 10587413,  
 10587706, 10587712, 10588106, 10588113, 10588306, 10588312, 10589206, 10589213, 10589306, 10589312, 10589506,  
 10589512, 10589606, 10589612, 10589706, 10589712, 10589906, 10589912, 10590212, 10590306, 10590312, 10590506,  
 10590512, 10590612, 10590717, 10590723, 10590806, 10590812, 10591006, 10591012, 10591305, 10591312, 10592006,  
 10592012, 10592502, 10592509, 10592606, 10592612, 10592705, 10592712, 10593006, 10593012, 10593205, 10593213,  
 10593505, 10593512, 10593806, 10593811, 10594205, 10594212, 10594305, 10594312, 10594405, 10594412, 10594505,  
 10594512, 10594605, 10594612, 10594804, 10595506, 10595512, 10596406, 10596505, 10596512, 10596603, 10596705,  
 10596713, 10596806, 10596812, 10596906, 10596912, 10597006, 10597012, 10597306, 10597312, 10597406, 10597412,  
 10598106, 10598112, 10598405, 10598412, 10598506, 10598511, 10598605, 10598612, 10598923, 10598929, 10599006,  
 10599013, 10599206, 10599212, 10599306, 10599312, 10599406, 10599412, 10600206, 10600213, 10600406, 10600412,  
 10600506, 10600514, 10600806, 10600812, 10600906, 10600912, 10601106, 10601114, 10601206, 10601212, 10601308,  
 10601314, 10601706, 10601712, 10601806, 10601812, 10602306, 10602312, 10602706, 10602712, 10602805, 10602906,  
 10602913, 10603006, 10603012, 10603306, 10603312, 10603406, 10603606, 10603612, 10603806, 10603812, 10604806,  
 10604812, 10605003, 10606206, 10606212, 10606406, 10606413, 10607003, 10607103, 10607109, 10607206, 10607212,  
 10607305, 10607312, 10607406, 10607412, 10607505, 10607512, 10607603, 10607705, 10607712, 10607806, 10607812,  
 10607905, 10607912, 10608002, 10608009, 10608305, 10608312, 10608405, 10608413, 10608605, 10608612, 10608905,  
 10608912, 10609005, 10609012, 10609205, 10609212, 10609305, 10609313, 10610206, 10610212, 10610506, 10610512,  
 10610606, 10610613, 10610706, 10610712, 10613706, 10613712, 10614103, 10615406, 10615412, 10615506, 10615512,  
 10615606, 10615612, 10615906, 10615912, 10616306, 10616312, 10616506, 10616512, 10616607, 10616612, 10616706,  
 10616712, 10616807, 10616815, 10616906, 10616912, 10617123, 10617129, 10617207, 10617214, 10617306, 10617314,  
 10618506, 10618512, 10619606, 10619806, 10619812, 10619906, 10619912, 10620006, 10620012, 10620106, 10620113,  
 10620206, 10620212, 10620406, 10620412, 10620506, 10620512, 10620806, 10620812, 10620906, 10620912, 10621606,  
 10621612, 10621706, 10621712, 10621806, 10621812, 10622006, 10622012, 10622106, 10622117, 10622206, 10622212,  
 10622312, 10622405, 10622412, 10622505, 10622514, 10622612, 10622905, 10622912, 10623805, 10623812, 10623905,  
 10623912, 10624706, 10624712, 10624906, 10624912, 10625006, 10625012, 10625106, 10625111, 10625303, 10625309,  
 10625403, 10625409, 10625520, 10625526, 10626306, 10626312, 10626506, 10626512, 10626606, 10626612, 10626906,

10626912, 10627006, 10627012, 10627206, 10627212, 10627306, 10627312, 10627407, 10627412, 10629103, 10629109,  
10630905, 10630912, 10631405, 10631412, 10631502, 10631509, 10631705, 10631712, 10632005, 10632012, 10633105,  
10633111, 10633206, 10633212, 10633505, 10633512, 10633706, 10633712, 10633806, 10633814, 10634006, 10634014,  
10634107, 10634112, 10634206, 10634212, 10634503, 10634509, 10634606, 10634612, 10634723, 10634729, 10636407,  
10636605, 10636612, 10636705, 10636712, 10636805, 10636812, 10636905, 10636913, 10637005, 10637012, 10637105,  
10637113, 10637205, 10637212, 10637706, 10637712, 10637806, 10637812, 10638305, 10638312, 10638405, 10638412,  
10638505, 10638512, 10638602, 10638609, 10639005, 10639012, 10639306, 10639312, 10639503, 10639509, 10639606,  
10639612, 10639706, 10639712, 10639806, 10639812, 10640003, 10640009, 10640106, 10640112, 10640206, 10640213,  
10640506, 10640512, 10640606, 10640612, 10640906, 10640912, 10643805, 10643812, 10643905, 10643911, 10644006,  
10644015, 10644806, 10644812, 10644907, 10644912, 10645003, 10645205, 10645212, 10645605, 10645612, 10645716,  
10645723, 10645805, 10645812, 10645905, 10645912, 10646006, 10647105, 10647112, 10647205, 10647212, 10647405,  
10647412, 10647503, 10647612, 10647705, 10647712, 10647905, 10647912, 10648005, 10648012, 10648823, 10648829,  
10648906, 10648912, 10649006, 10649012, 10649806, 10649812, 10650006, 10650012, 10650106, 10650112, 10651305,  
10651313, 10651405, 10651412, 10651805, 10651812, 10651905, 10651912, 10652005, 10652012, 10653105, 10653112,  
10653305, 10653312, 10653405, 10653412, 10653623, 10653629, 10653706, 10653712, 10653823, 10653829, 10654106,  
10654112, 10654206, 10654212, 10656723, 10656729, 10656803, 10658706, 10658712, 10658812, 10659206, 10659212,  
10659306, 10659312, 10659405, 10659412, 10659505, 10659512, 10659905, 10659912, 10660107, 10660112, 10660405,  
10660412, 10660605, 10660612, 10660705, 10660712, 10661103, 10661109, 10661903, 10661909, 10662006, 10662012,  
10662106, 10662112, 10662209, 10662303, 10662309, 10662506, 10662512, 10662606, 10662612, 10662806, 10662814,  
10662906, 10662912, 10663023, 10663029, 10663203, 10663209, 10663306, 10663312, 10663506, 10663512, 10663606,  
10663612, 10663706, 10663712, 10667006, 10667012, 10668006, 10668012, 10668206, 10668212, 10668306, 10668312,  
10668403, 10669706, 10669712, 10669806, 10669812, 10669906, 10669911, 10670505, 10670512, 10670605, 10670612,  
10674005, 10674011, 10674105, 10674112, 10674205, 10674211, 10674331, 10674337, 10674405, 10674411, 10674605,  
10674611, 10674721, 10674727, 10675005, 10675011, 10675105, 10675113, 10675405, 10675411, 10675505, 10675511,  
10675905, 10675913, 10676006, 10676012, 10676408, 10676412, 10676521, 10676527, 10676606, 10676612, 10676705,  
10676711, 10676905, 10676911, 10677005, 10677011, 10677105, 10677111, 10677205, 10677211, 10677505, 10677511,  
10677603, 10677609, 10677803, 10677906, 10677912, 10678005, 10678011, 10678205, 10678211, 10678303, 10678311,  
10678506, 10678512, 10678603, 10678609, 10678803, 10678809, 10678905, 10678911, 10679005, 10679011, 10679105,  
10679111, 10679205, 10679211, 10679306, 10679313, 10679605, 10679611, 10679805, 10679812, 10679905, 10679911,  
10680003, 10680009, 10680103, 10680109, 10680406, 10680415, 10680505, 10680511, 10680606, 10680612, 10680703,  
10680709, 10680905, 10680911, 10681105, 10681111, 10681202, 10681320, 10681326, 10681705, 10681711, 10681806,  
10681812, 10681905, 10681911, 10682006, 10682013, 10682105, 10682111, 10682206, 10682212, 10682305, 10682311,  
10682505, 10682512, 10682605, 10682611, 10682905, 10682911, 10683021, 10683027, 10683106, 10683112, 10683205,  
10683211, 10683306, 10683312, 10683506, 10683512, 10683605, 10683611, 10683706, 10683712, 10683906, 10683912,  
10684106, 10684114, 10684203, 10684209, 10684705, 10684711, 10684805, 10684811, 10684903, 10684909, 10685005,  
10685011, 10685405, 10685413, 10685503, 10685703, 10685806, 10685812, 10686006, 10686305, 10686311, 10686905,  
10686911, 10687105, 10687111, 10687906, 10687912, 10688106, 10688112, 10688206, 10688212, 10688406, 10688412,  
10688506, 10688512, 10688606, 10688612, 10688706, 10688712, 10688806, 10688812, 10688907, 10689006, 10689012,  
10689123, 10689129, 10689206, 10689212, 10689406, 10689412, 10690103, 10690111, 10690205, 10690211, 10690405,  
10690411, 10690505, 10690511, 10690705, 10690711, 10690905, 10690911, 10691023, 10691029, 10691206, 10691305,  
10691314, 10691423, 10691503, 10691509, 10691705, 10691711, 10692004, 10692011, 10692103, 10692109, 10692205,  
10692216, 10692406, 10692413, 10692506, 10692517, 10692906, 10692911, 10693205, 10693212, 10693306, 10693312,  
10693406, 10693525, 10693531, 10693606, 10693612, 10693706, 10693712, 10693806, 10694006, 10694014, 10694106,  
10694112, 10694206, 10694212, 10694303, 10694309, 10694406, 10694412, 10694506, 10694512, 10694606, 10694611,  
10694706, 10694712, 10694809, 10694906, 10694912, 10695206, 10695212, 10695406, 10695412, 10695504, 10695703,

10695803, 10695809, 10695906, 10695913, 10696106, 10696112, 10696206, 10696213, 10696306, 10696312, 10696406,  
 10696412, 10696603, 10696609, 10696706, 10696712, 10696803, 10696809, 10696933, 10696938, 10697006, 10697012,  
 10697206, 10697212, 10697303, 10697406, 10697412, 10697606, 10697613, 10697703, 10697709, 10697803, 10697810,  
 10697906, 10697913, 10698006, 10698014, 10698103, 10698109, 10698206, 10698212, 10698406, 10698412, 10698503,  
 10698509, 10698606, 10698612, 10698840, 10698846, 10698906, 10698912, 10699123, 10699129, 10699258, 10699303,  
 10699309, 10699403, 10699409, 10699506, 10699513, 10699603, 10699609, 10699722, 10699731, 10699906, 10699913,  
 10700106, 10700114, 10700206, 10700214, 10700406, 10700412, 10700703, 10700709, 10700906, 10700912, 10701006,  
 10701012, 10701103, 10701109, 10701206, 10701212, 10701306, 10701312, 10701406, 10701412, 10702006, 10702012,  
 10702206, 10702212, 10702406, 10702412, 10702506, 10702514, 10702606, 10702612, 10702706, 10702712, 10702823,  
 10702829, 10702906, 10702914, 10703006, 10703013, 10703306, 10703313, 10703423, 10703429, 10703524, 10703531,  
 10703706, 10703720, 10703806, 10703812, 10704006, 10704012, 10704106, 10704112, 10704207, 10704212, 10704306,  
 10704312, 10704406, 10704412, 10704506, 10704512, 10704603, 10704706, 10704712, 10704806, 10704813, 10705003,  
 10705406, 10705412, 10705523, 10705529, 10705603, 10705706, 10705712, 10705806, 10705812, 10705906, 10705912,  
 10706223, 10706230, 10706306, 10706312, 10706403, 10706409, 10706706, 10706712, 10706806, 10706812, 10707006,  
 10707013, 10710003, 10710105, 10710112, 10710203, 10710213, 10710403, 10710409, 10710505, 10710512, 10710904,  
 10711112, 10711206, 10711212, 10711406, 10711411, 10711706, 10711712, 10711806, 10711812, 10712006, 10712012,  
 10712106, 10712113, 10712206, 10712212, 10712406, 10712412, 10712506, 10712513, 10712607, 10712613, 10712705,  
 10712712, 10713006, 10713012, 10713123, 10713129, 10713206, 10713212, 10713306, 10713312, 10713406, 10713413,  
 10713505, 10713512, 10713606, 10713613, 10713905, 10713912, 10714105, 10714112, 10714206, 10714212, 10714423,  
 10714429, 10714522, 10714531, 10714603, 10714705, 10714712, 10714905, 10714914, 10715305, 10715312, 10715505,  
 10715513, 10715604, 10715610, 10715706, 10715712, 10715806, 10715812, 10715906, 10715912, 10716003, 10716105,  
 10716113, 10716306, 10716312, 10716403, 10716507, 10716513, 10716603, 10716806, 10716813, 10716906, 10716912,  
 10717006, 10717012, 10717106, 10717112, 10717212, 10717306, 10717312, 10717706, 10717712, 10717806, 10717812,  
 10717923, 10717929, 10718006, 10718012, 10718106, 10718112, 10718205, 10718212, 10718506, 10718512, 10718706,  
 10718712, 10718805, 10718814, 10718906, 10718912, 10719105, 10719114, 10719203, 10719209, 10719302, 10719311,  
 10719505, 10719512, 10719606, 10719612, 10719806, 10719812, 10719905, 10719912, 10720006, 10720012, 10720206,  
 10720213, 10720305, 10720313, 10720442, 10720448, 10720505, 10720512, 10720606, 10720612, 10720806, 10720812,  
 10720906, 10720912, 10721105, 10721113, 10721205, 10721212, 10721305, 10721312, 10721605, 10721612, 10721708,  
 10721712, 10721905, 10721912, 10722006, 10722012, 10722208, 10722213, 10722503, 10722509, 10722606, 10722612,  
 10722706, 10722712, 10722805, 10722812, 10722906, 10722912, 10723005, 10723012, 10723103, 10723109, 10723306,  
 10723313, 10723405, 10723412, 10723706, 10723715, 10723805, 10723813, 10723906, 10723912, 10724005, 10724013,  
 10724106, 10724112, 10724205, 10724212, 10724405, 10724506, 10724514, 10724706, 10724712, 10724805, 10724812,  
 10724906, 10724912, 10725203, 10725306, 10725312, 10725403, 10725506, 10725512, 10725706, 10725712, 10725806,  
 10725812, 10726006, 10726013, 10726106, 10726112, 10726306, 10726312, 10726405, 10726412, 10726506, 10726512,  
 10726606, 10726612, 10726906, 10726912, 10727306, 10727312, 10727406, 10727412, 10727506, 10727512, 10727606,  
 10727612, 10727706, 10727712, 10727806, 10728006, 10728014, 10728106, 10728112, 10728306, 10728312, 10728406,  
 10728412, 10728606, 10728612, 10728706, 10728712, 10728803, 10728809, 10728908, 10728913, 10729006, 10729012,  
 10729106, 10729112, 10729207, 10729213, 10729306, 10729313, 10729603, 10729705, 10729712, 10729806, 10729812,  
 10730006, 10730012, 10730106, 10730114, 10730505, 10730512, 10730606, 10730614, 10730905, 10730912, 10731005,  
 10731012, 10731106, 10731112, 10731205, 10731214, 10731306, 10731312, 10731405, 10731415, 10731506, 10731512,  
 10731706, 10731713, 10731808, 10731818, 10731906, 10731913, 10732006, 10732012, 10732106, 10732112, 10732203,  
 10732211, 10732406, 10732412, 10732608, 10732614, 10732726, 10732732, 10733306, 10733313, 10733406, 10733412,  
 10733506, 10733512, 10733606, 10733612, 10733706, 10733712, 10733806, 10733812, 10733906, 10733912, 10734006,  
 10734012, 10734105, 10734113, 10734206, 10734212, 10734406, 10734412, 10734505, 10734512, 10734606, 10734612,  
 10734806, 10734812, 10734905, 10734912, 10735106, 10735113, 10735206, 10735213, 10735306, 10735312, 10735405,



10735412, 10735506, 10735512, 10735604, 10735720, 10735726, 10736005, 10736012, 10736202, 10736210, 10736405,  
10736412, 10736768, 10736774, 10736805, 10736812, 10736906, 10736912, 10737022, 10737029, 10737103, 10737405,  
10737413, 10737706, 10737712, 10737906, 10737912, 10738003, 10738106, 10738112, 10738228, 10738235, 10738306,  
10738314, 10738606, 10738612, 10738706, 10738712, 10738805, 10738812, 10739005, 10739012, 10739208, 10739302,  
10739309, 10739406, 10739413, 10739523, 10739529, 10739605, 10739612, 10739706, 10739712, 10740012, 10740113,  
10740223, 10740229, 10740304, 10740423, 10740430, 10740506, 10740512, 10740606, 10740611, 10740706, 10740712,  
10740806, 10740812, 10740906, 10740912, 10741006, 10741012, 10741205, 10741212, 10741407, 10741412, 10742312,  
10742606, 10742612, 10742706, 10742712, 10743017, 10743107, 10743209, 10743215, 10743305, 10743314, 10743640,  
10743646, 10743805, 10743812, 10743905, 10743912, 10744005, 10744012, 10744222, 10744229, 10744305, 10744312,  
10744605, 10744612, 10744705, 10744712, 10744805, 10744813, 10744905, 10744912, 10745005, 10745012, 10745105,  
10745112, 10745207, 10745213, 10745305, 10745312, 10745424, 10745429, 10745505, 10745513, 10745605, 10745612,  
10745706, 10745713, 10745903, 10746006, 10746012, 10746106, 10746112, 10746223, 10746229, 10746306, 10746312,  
10746440, 10746446, 10746709, 10746815, 10746822, 10746906, 10746912, 10747103, 10747110, 10747306, 10747312,  
10747506, 10747513, 10747806, 10747812, 10747906, 10747912, 10748006, 10748012, 10748106, 10748112, 10748206,  
10748212, 10748306, 10748312, 10748403, 10748409, 10748606, 10748613, 10748706, 10748712, 10748806, 10748812,  
10749106, 10749112, 10749206, 10749212, 10749306, 10749312, 10749406, 10749413, 10749506, 10749512, 10749706,  
10749712, 10749806, 10749812, 10750106, 10750112, 10750206, 10750212, 10750322, 10750329, 10750406, 10750412,  
10750606, 10750612, 10750806, 10750812, 10750922, 10750929, 10751003, 10751009, 10751139, 10751147, 10751305,  
10751313, 10751502, 10751509, 10751905, 10751912, 10752005, 10752012, 10752205, 10752212, 10752405, 10752412,  
10752622, 10752630, 10752708, 10752715, 10752908, 10752915, 10753006, 10753012, 10753208, 10753213, 10753308,  
10753314, 10753406, 10753412, 10753508, 10753515, 10753626, 10753631, 10753726, 10753734, 10753829, 10753840,  
10753905, 10753912, 10754009, 10754015, 10754226, 10754322, 10754329, 10754449, 10754643, 10754649, 10754702,  
10754926, 10754932, 10755323, 10755329, 10755406, 10755412, 10755640, 10755646, 10755717, 10755803, 10755809,  
10756006, 10756013, 10756324, 10756330, 10756406, 10756412, 10756606, 10756612, 10756723, 10756729, 10756806,  
10756812, 10757003, 10757009, 10757440, 10757446, 10757640, 10757646, 10757706, 10757713, 10757908, 10757914,  
10758023, 10758029, 10758105, 10758113, 10758223, 10758229, 10758305, 10758312, 10758505, 10758512, 10758623,  
10758629, 10758705, 10758712, 10758803, 10758809, 10758905, 10758913, 10759023, 10759029, 10759105, 10759112,  
10759223, 10759229, 10759305, 10759312, 10759606, 10759612, 10759705, 10759712, 10759807, 10759813, 10759937,  
10759944, 10760006, 10760012, 10760102, 10760109, 10760306, 10760312, 10760422, 10760429, 10760706, 10760712,  
10760906, 10760912, 10761205, 10761212, 10761324, 10761330, 10761605, 10761612, 10761724, 10761730, 10761805,  
10761813, 10761905, 10761912, 10762005, 10762012, 10762103, 10762109, 10762222, 10762230, 10762505, 10762512,  
10762605, 10762612, 10762705, 10762712, 10762806, 10762812, 10762905, 10762912, 10763105, 10763112, 10763206,  
10763212, 10763705, 10763712, 10763922, 10763929, 10764006, 10764012, 10764123, 10764129, 10764206, 10764212,  
10764406, 10764412, 10764506, 10764512, 10764606, 10764612, 10764706, 10764712, 10764827, 10764833, 10764923,  
10764929, 10765106, 10765112, 10765206, 10765212, 10765406, 10765412, 10765505, 10765512, 10765705, 10765712,  
10765806, 10765812, 10765906, 10765912, 10766206, 10766213, 10766306, 10766312, 10766406, 10766412, 10766506,  
10766512, 10766913, 10767005, 10767012, 10767106, 10767112, 10767205, 10767212, 10767405, 10767412, 10767706,  
10767712, 10767940, 10767946, 10768206, 10768212, 10768306, 10768312, 10768606, 10768612, 10768706, 10768712,  
10768825, 10768832, 10769006, 10769012, 10769106, 10769112, 10769206, 10769212, 10769406, 10769412, 10769606,  
10769612, 10769706, 10769712, 10769806, 10769812, 10769906, 10769913, 10770406, 10770412, 10770603, 10770609,  
10770724, 10770730, 10770824, 10770830, 10770906, 10770913, 10771006, 10771012, 10771105, 10771112, 10771206,  
10771212, 10771406, 10771412, 10771623, 10771629, 10771705, 10771712, 10771806, 10771812, 10771922, 10771929,  
10772006, 10772108, 10772203, 10772606, 10772613, 10772806, 10772812, 10772906, 10772912, 10773306, 10773313,  
10773506, 10773512, 10773606, 10773614, 10773806, 10773812, 10774406, 10774412, 10774506, 10774512, 10774706,  
10774712, 10775106, 10775112, 10775306, 10775312, 10775406, 10775412, 10776605, 10776612, 10777106, 10777606,

10777612, 10777703, 10777806, 10777812, 10777906, 10777912, 10778006, 10778012, 10778106, 10778112, 10778203,  
 10778211, 10778406, 10778413, 10778606, 10778612, 10779306, 10779312, 10779603, 10779906, 10780006, 10780012,  
 10780205, 10780212, 10780306, 10780312, 10780405, 10780412, 10780506, 10780512, 10780605, 10780612, 10780706,  
 10780712, 10780906, 10780912, 10781123, 10781129, 10781312, 10781503, 10781511, 10781706, 10781712, 10781822,  
 10781829, 10782506, 10782512, 10782806, 10782812, 10782903, 10782909, 10783306, 10783312, 10783706, 10783712,  
 10784107, 10784114, 10784303, 10784309, 10785005, 10785012, 10785205, 10785212, 10785605, 10785612, 10785706,  
 10785712, 10785805, 10785812, 10786106, 10786112, 10786205, 10786212, 10786306, 10786312, 10786405, 10786412,  
 10786706, 10786712, 10787006, 10787012, 10787706, 10787712, 10788106, 10788112, 10788306, 10788312, 10788512,  
 10788706, 10788712, 10788806, 10788812, 10789212, 10789506, 10789512, 10789706, 10789712, 10789905, 10789912,  
 10790105, 10790112, 10790705, 10790712, 10791005, 10791013, 10791106, 10791113, 10791305, 10791312, 10791406,  
 10791412, 10791506, 10791512, 10791706, 10792306, 10792312, 10792706, 10792712, 10792806, 10792812, 10793106,  
 10793112, 10793406, 10793414, 10793506, 10793512, 10793606, 10793612, 10794105, 10794112, 10794305, 10794312,  
 10794406, 10794412, 10794922, 10794929, 10795805, 10795813, 10796205, 10796212, 10797306, 10797312, 10798005,  
 10798012, 10798405, 10798412, 10798806, 10798813, 10800306, 10800312, 10800406, 10800412, 10800523, 10800529,  
 10800906, 10800913, 10801107, 10801113, 10801506, 10801512, 10801706, 10801712, 10801905, 10801912, 10802623,  
 10802629, 10802823, 10802829, 10802905, 10802912, 10803106, 10803112, 10803206, 10803212, 10803506, 10803512,  
 10803606, 10803612, 10803706, 10803716, 10803806, 10803811, 10804106, 10804112, 10804306, 10804312, 10804606,  
 10804612, 10804706, 10804712, 10806006, 10806012, 10806106, 10806114, 10806206, 10806212, 10806306, 10806312,  
 10806505, 10806512, 10807705, 10807712, 10808005, 10808012, 10808505, 10808512, 10811003, 10811106, 10811112,  
 10811206, 10811212, 10815405, 10815412, 10816505, 10817006, 10817014, 10817112, 10817206, 10817212, 10817306,  
 10817312, 10817506, 10817512, 10817606, 10817612, 10817706, 10817712, 10818706, 10818712, 10818906, 10818912,  
 10819106, 10819112, 10819206, 10819212, 10819606, 10819612, 10821406, 10821412, 10821506, 10821512, 10825305,  
 10826005, 10826012, 10827105, 10827111, 10827206, 10827214, 10827306, 10827312, 10827606, 10827612, 10827706,  
 10827712, 10827806, 10827812, 10827906, 10827912, 10828506, 10828512, 10828606, 10828707, 10828713, 10828803,  
 10828815, 10828906, 10828912, 10833206, 10833212, 10833406, 10833412, 10833506, 10833512, 10833606, 10833612,  
 10836006, 10836012, 10836206, 10836211, 10836406, 10836412, 10836706, 10836712, 10836903, 10836909, 10837506,  
 10837512, 10837706, 10837712, 10838003, 10838009, 10838106, 10838112, 10841405, 10844040, 10844403, 10844409,  
 10845003, 10845009, 10845412, 10845606, 10845612, 10846203, 10846209, 10846606, 10846613, 10846806, 10846813,  
 10847106, 10847112, 10847206, 10847212, 10847706, 10847712, 10847803, 10847812, 10848106, 10848112, 10848303,  
 10848309, 10848403, 10848606, 10848612, 10851103, 10851109, 10851306, 10851312, 10851903, 10851909, 10852206,  
 10852212, 10852506, 10852512, 10853103, 10853109, 10853606, 10853612, 10853806, 10854006, 10854012, 10854106,  
 10854112, 10856306, 10856312, 10858903, 10858910, 10861206, 10861212, 10861306, 10861312, 10861406, 10861412,  
 10861706, 10861712, 10861806, 10861812, 10862306, 10862312, 10864203, 10864209, 10867303, 10867503, 10867509,  
 10868106, 10868112, 10868306, 10868312, 10868505, 10868512, 10868623, 10868629, 10869206, 10869212, 10869606,  
 10869612, 10869703, 10869709, 10870406, 10870412, 10870506, 10870512, 10870603, 10870609, 10870706, 10870713,  
 10870906, 10870912, 10871006, 10871012, 10871106, 10873903, 10873909, 10874303, 10874309, 10874506, 10874512,  
 10874706, 10874712, 10874906, 10874912, 10875223, 10875230, 10879206, 10879212, 10879306, 10879312, 10879406,  
 10879412, 10879503, 10879509, 10880106, 10880112, 10880206, 10880212, 10880306, 10880312, 10880506, 10880513,  
 10880607, 10880612, 10881709, 10882206, 10882212, 10882306, 10882312, 10882506, 10882512, 10882606, 10882612,  
 10883006, 10883013, 10883406, 10883412, 10883506, 10883512, 10883606, 10883612, 10883706, 10883712, 10883903,  
 10883911, 10884006, 10884012, 10884106, 10884112, 10884203, 10884209, 10884303, 10884309, 10885603, 10885609,  
 10886207, 10886213, 10886306, 10886312, 10889903, 10889909, 10890006, 10890012, 10890106, 10890112, 10890206,  
 10890212, 10890506, 10890512, 10890706, 10890712, 10892703, 10892709, 10893107, 10893112, 10893206, 10893212,  
 10893306, 10893312, 10893606, 10893612, 10893706, 10893712, 10893807, 10893812, 10894403, 10894409, 10894906,  
 10894912, 10895006, 10895012, 10895106, 10895112, 10895303, 10895309, 10895706, 10895713, 10899222, 10899228,

10899406, 10899412, 10899606, 10899612, 10899806, 10899812, 10899906, 10899912, 10902606, 10902612, 10903703, 10903806, 10903812, 10903906, 10903912, 10904109, 10904114, 10904203, 10904306, 10904312, 10904906, 10904912, 10905106, 10905112, 10905211, 10905307, 10905312, 10905506, 10905512, 10905606, 10905612, 10905806, 10905812, 10906203, 10906209, 10906403, 10906409, 10906602, 10906609, 10908506, 10908512, 10908606, 10908612, 10908806, 10908812, 10911803, 10912106, 10912112, 10912206, 10912212, 10912507, 10912513, 10912606, 10912612, 10912706, 10912712, 10912903, 10912909, 10913303, 10913309, 10914806, 10914812, 10914906, 10914912, 10915003, 10915009, 10915206, 10915212, 10917006, 10917012, 10917106, 10917112, 10917306, 10917312, 10917404, 10917410, 10917506, 10917512, 10917603, 10917609, 10920706, 10921003, 10921009, 10921106, 10921112, 10922006, 10922012, 10922406, 10922412, 10922503, 10922509, 10922906, 10922912, 10923206, 10923212, 10923305, 10923312, 10923406, 10923412, 10923705, 10923712, 10923907, 10923912, 10924205, 10924213, 10924306, 10924312, 10924405, 10924412, 10924523, 10924529, 10924706, 10924712, 10924805, 10924811, 10925306, 10925312, 10925506, 10925512, 10925906, 10925912, 10926205, 10926212, 10926503, 10927006, 10927012, 10927206, 10927212, 10927406, 10927412, 10927506, 10927512, 10927606, 10928506, 10928512, 10928606, 10928612, 10928806, 10928812, 10928906, 10928912, 10929006, 10929012, 10929106, 10929112, 10929206, 10929212, 10929306, 10929312, 10929506, 10929512, 10929703, 10929709, 10929806, 10929812, 10930006, 10930012, 10930206, 10930213, 10930313, 10930406, 10930412, 10930606, 10930613, 10930706, 10930712, 10930906, 10930913, 10931306, 10931312, 10931423, 10931429, 10931506, 10931513, 10931606, 10931612, 10931706, 10931712, 10931806, 10931812, 10931906, 10931914, 10932005, 10932012, 10932106, 10932112, 10932205, 10932212, 10932606, 10932612, 10932707, 10932716, 10932806, 10932812, 10933305, 10933312, 10933606, 10933612, 10934006, 10934012, 10934106, 10934112, 10934206, 10934212, 10934506, 10934512, 10934603, 10934609, 10934706, 10934712, 10934806, 10934812, 10934906, 10934912, 10935005, 10935012, 10935305, 10935312, 10935405, 10935412, 10935605, 10935612, 10935705, 10935712, 10935805, 10935812, 10935905, 10935912, 10936005, 10936012, 10936502, 10936510, 10936606, 10936612, 10936705, 10936714, 10936812, 10936905, 10936912, 10937304, 10937506, 10937512, 10938106, 10938114, 10938406, 10938412, 10938606, 10938614, 10938706, 10938712, 10938806, 10938812, 10939006, 10939012, 10939219, 10939225, 10939606, 10939612, 10939706, 10939712, 10939906, 10939912, 10940003, 10940009, 10940406, 10940412, 10940606, 10940612, 10940806, 10940812, 10940906, 10940912, 10941003, 10941106, 10941112, 10941406, 10941412, 10942205, 10942213, 10942408, 10942413, 10943005, 10943012, 10943306, 10943312, 10943405, 10943412, 10943805, 10943812, 10943906, 10943912, 10944805, 10944812, 10945006, 10945105, 10945112, 10945206, 10945212, 10945305, 10945312, 10945705, 10945712, 10945905, 10945912, 10946406, 10946412, 10946505, 10946512, 10946705, 10946712, 10947006, 10947013, 10947106, 10947112, 10947205, 10947212, 10947306, 10947313, 10947805, 10947812, 10948006, 10948012, 10948206, 10948212, 10948306, 10948312, 10948406, 10948412, 10948606, 10949003, 10949106, 10949112, 10949806, 10949812, 10949906, 10949912, 10950106, 10950112, 10950306, 10950312, 10950523, 10950529, 10950706, 10950712, 10951103, 10951306, 10951313, 10951406, 10951412, 10951706, 10951712, 10951906, 10951912, 10952106, 10952112, 10952305, 10952406, 10952413, 10952605, 10952611, 10953006, 10953012, 10953106, 10953114, 10953306, 10953312, 10953506, 10953512, 10954006, 10954012, 10954205, 10954703, 10954806, 10954812, 10955105, 10955113, 10955203, 10955209, 10955305, 10955312, 10955505, 10955511, 10955606, 10955614, 10955721, 10955728, 10956005, 10956012, 10956105, 10956113, 10956305, 10956312, 10956405, 10956412, 10956605, 10956612, 10956805, 10956812, 10957004, 10957105, 10957112, 10957405, 10957412, 10957505, 10957512, 10957605, 10957612, 10958205, 10958212, 10958305, 10958312, 10958405, 10958412, 10958505, 10958512, 10958905, 10958912, 10959003, 10959009, 10959203, 10959209, 10959505, 10959512, 10961506, 10961512, 10961706, 10961712, 10968103, 10968109, 10974103, 10974109, 11073206, 11073212, 11073603, 11073609, 11074103, 11074109, 11075303, 11075309, 11075407, 11075413, 11075606, 11075612, 11075903, 11076009, 11076106, 11076113, 11076206, 11076213, 11076403, 11076409, 11081506, 11081512, 11081806, 11081812, 11081906, 11081912, 11085703, 11085709, 11085806, 11085812, 11086240, 11086306, 11086312, 11088109, 11088606, 11088612, 11088703, 11088709, 11090106, 11090112, 11090206, 11090212, 11090806, 11090812, 11090906, 11090912, 11091223, 11091229, 11091303, 11092803, 11092809, 11094406, 11094412, 11094603, 11094706, 11094712, 11096206, 11096212, 11096306, 11096312, 11096508, 11096515, 11096606, 11096612,

11096706, 11096715, 11096806, 11096812, 11100012, 11101606, 11101612, 11101706, 11101712, 11101806, 11101812, 11102206, 11102212, 11102303, 11102803, 11102809, 11103306, 11103312, 11103403, 11103606, 11103612, 11103803, 11103809, 11105503, 11105509, 11108503, 11108509, 11109006, 11109012, 11109206, 11109212, 11109606, 11109612, 11110003, 11110009, 11110306, 11110312, 11110806, 11110812, 11110912, 11111003, 11111009, 11112003, 11112009, 11116606, 11116612, 11116706, 11116712, 11118806, 11118812, 11119006, 11119012, 11119306, 11119312, 11119407, 11119412, 11121706, 11121712, 11121906, 11121912, 11123703, 11123709, 11126403, 11126409, 11126906, 11126912, 11127006, 11127012, 11128706, 11128712, 11128806, 11128812, 11128906, 11128912, 11131803, 11131809, 11133003, 11133009, 11134103, 11134109, 11134606, 11134612, 11134706, 11134712, 11135103, 11135206, 11135212, 11135303, 11135503, 11135509, 11135706, 11135712, 11135906, 11135912, 11136006, 11136012, 11136106, 11136112, 11137103, 11137109, 11137317, 11137323, 11137806, 11137813, 11137906, 11137912, 11138103, 11138109, 11139006, 11139012, 11140023, 11140029, 11140206, 11140212, 11141005, 11141012, 11141506, 11141514, 11142106, 11142223, 11142229, 11143003, 11143009, 11145303, 11145309, 11145703, 11145709, 11145902, 11145909, 11146303, 11146309, 11147523, 11147530, 11147606, 11147612, 11147706, 11147712, 11152003, 11152009, 11153603, 11153609, 11154103, 11154109, 11154703, 11154709, 11154903, 11154909, 11160903, 11160909, 11161003, 11161009, 11162323, 11162329, 11164006, 11164012, 11165206, 11165212, 11165506, 11165806, 11165812, 11165906, 11165912, 11168903, 11168909, 11173003, 11173009, 11174406, 11174412, 11175907, 11175912, 11176703, 11176709, 11177103, 11177109, 11177906, 11177912, 11178006, 11178012, 11180303, 11180309, 11186503, 11186509, 11190906, 11190912, 11191123, 11191129, 11191206, 11191212, 11192803, 11192809, 11193803, 11193809, 11201003, 11201009, 11202103, 11202109, 11202303, 11202309, 11203003, 11203009, 11213203, 11213209, 11213303, 11213309, 11213803, 11213809, 11214103, 11214109, 11215203, 11215209, 11217903, 11217909, 11218303, 11218309, 11218903, 11218909, 11221903, 11221909, 11227017, 11227023, 11227803, 11227809, 11228303, 11228309, 11235803, 11235809, 11243103, 11243109, 11243903, 11243909, 11244303, 11244309, 11244403, 11244409, 11244703, 11244709, 11244803, 11244809, 11245503, 11245509, 11246403, 11246409, 11250803, 11250809, 11251303, 11251309, 11252503, 11252509, 11258103, 11258109, 11304203, 11304209, 11326412, 11326418, 11334617, 11334623, 11336703, 11336709, 11348609

## References

1. Peterfy, C., Gold, G., Eckstein, F., Cicuttini, F., Dardzinski, B., Stevens, R.: MRI protocols for whole-organ assessment of the knee in osteoarthritis. Osteoarthritis and cartilage **14**, 95–111 (2006)
